# Supplementary material for: Comparison of Bayesian methods for extrapolation of treatment effects: a simulation study
Source: arXiv:2504.01949 source file (2026-10-15)
Supplement: Supplementary file 1 [file supplementary.tex]

\documentclass[./paper.tex]{subfiles} 
\begin{document}

\appendix 
\section*{Supplementary material}
\label{appendix}
\renewcommand{\thefigure}{S\arabic{figure}}
\renewcommand{\thetable}{S\arabic{table}}

% Reset figure and table counters
\setcounter{figure}{0}
\setcounter{table}{0}

\section{Supplementary methods}
 \subsection{Definition of the drift ranges}
 \label{supp:definition_drift_ranges}
However, with an adaptive borrowing method,  the probability of meeting the decision criterion, $\operatorname{Pr}(\text{Study success}|\mathbf{D}_T = d_T, \mathbf{D}_S= d_S)$, is expected to reach a maximum at some drift value beyond which source data starts being discarded. For the study of adaptive borrowing methods, it is thus important to select a range of drift wide enough for this discarding phenomenon to be observed.

To determine the range of drift to consider for a given case study, we propose the following rationale when the likelihood is Gaussian: one may consider that if the overlap between the posterior distribution of the treatment effect in the source study $p(\theta_S|\mathbf{y}_S)$ and the target study $p(\theta_T|\mathbf{y}_T)$ is very small, the source study should be discarded. To include this idea in our simulation framework, we analytically determined, for a given value of $\theta_T = \hat{\theta}_S + \delta$, the Hellinger distance between $\mathcal{N}\left(\hat{\theta}_S, \sigma^2_{\theta_S}\right)$, where $\sigma_{\theta_S}$ is the standard error on $\theta_S$, and  $\mathcal{N}\left(\hat{\theta}_S + \delta, \sigma^2_{\theta_T}\right)$, where $\sigma_{\theta_T}$ is the standard error on $\theta_T$ derived from the observed target study data alone. 
%The Hellinger distance $H(f,g)$ between two probability distributions $f$ and $g$ is defined %as : 
%$$H^2(f, g)=\frac{1}{2} \int(\sqrt{f(x)}-\sqrt{g(x)})^2 d x=1-\int \sqrt{f(x) g(x)} d x$$
 
We determined the value of the negative drift for which the Hellinger distance reaches 0.9, and used this as the lower boundary of the drift ranges considered. Beyond such an extreme value for the observed drift, borrowing from source data can be considered futile.
Note that, for simplicity, we used the same drift range for all scenarios in a given case study, irrespective of later changes introduced in the denominator of source ratio-like summary measures or target study sampling standard deviation.

Note that in cases where the posterior predictive $p(\overline{y}_T|\theta_T,\sigma^2_{\theta_T})$ is very wide, it may not be guaranteed that the range $[\theta_0 - \hat{\theta}_S, 0]$ is included within the drift range obtained with the above method (noted $\mathscr{R}$). Although this case may happen in very rare cases given the quite conservative threshold of 0.9 considered, we used the range $\mathscr{R} \cup [\theta_0 - \hat{\theta}_S, 0]$ for the drift in practice. We observed that  $[\theta_0 - \hat{\theta}_S, 0] \subset  \mathscr{R}$  in all case studies considered.

When the treatment effect is a difference of rates,  $\theta_T = p_T^{(t)} - p_T^{(c)}$, where $p_T^{(a)}$ is the response rate in arm $a$ of the target trial,  $\theta_T$ spans the range $[-1,1]$. Therefore the drift spans the interval $[-1-\hat{\theta}_S,1-\hat{\theta}_S]$. Moreover, we need to ensure that $p_T^{(t)}$ and $p_T^{(c)}$ are within $[0,1]$. Since we assume $p_T^{(c)} = \hat{p}_S^{(c)}$, we have:
 
$p_T^{(t)} = \theta_T + p_T^{(c)} = \delta + \hat{\theta}_S + \hat{p}_S^{(c)}  = \delta + \hat{p}_S^{(t)}$
This implies the following constraint: $  -\hat{p}_S^{(t)} \leq \delta  \leq 1 - \hat{p}_S^{(t)}$. By combining these two constraints, the drift interval is $\mathscr{R} = [\operatorname{max}(-1-\hat{\theta}_S, -\hat{p}_S^{(t)}), \operatorname{min}(1-\hat{\theta}_S,  1 - \hat{p}_S^{(t)})]$. 

The corresponding drift ranges considered for each case study are listed in Supplementary Table \ref{tab:drift_ranges}. We considered evenly spaced values in the range of drift. Note that, for computational cost reasons, we did not use the same number of drift values for each method and each case study. 

\subsection{Normalized Power Prior}

\label{supp:normalized_power_prior}
\textcite{pawel_normalized_2023}  or in appendix A of \textcite{gravestock_adaptive_2017}. In this setting, the normalized power prior is: 

$$
\pi\left(\theta_T, \gamma \mid \mathbf{D}_S\right)=\frac{\mathcal{L}\left(\mathbf{D}_S \mid \theta_T\right)^\gamma \pi(\gamma)}{\int_{-\infty}^{+\infty} \mathcal{L}\left(\mathbf{D}_S \mid \theta_T^{\prime}\right)^\gamma d \theta_T^{\prime}}=\mathcal{N}\left(\theta_T \mid \hat{\theta}_S, \sigma_{\theta_S}^2 / \gamma\right) \operatorname{Be}(\gamma \mid p, q)
$$
The marginal prior on $\theta_T$ is :

\begin{equation}
\begin{aligned}
\pi\left(\theta_T\mid \mathbf{D}_S\right) &= \int_0^1 \mathcal{N}\left(\theta_T \mid \hat{\theta}_S, \sigma_{\theta_S}^2 / \gamma\right) \operatorname{Be}(\gamma \mid p, q)d\gamma \\
%& = \frac{1}{\mathrm{~B}(p, q)} \frac{1}{\sqrt{2 \pi \sigma_{\theta_S}^2}} \int_0^1 \sqrt{\gamma} \operatorname{exp}\left(\gamma \frac{\left(\hat{\theta}_S-\theta_T\right)^2}{-2 \sigma_{\theta_S}^2}\right) \gamma^{p-1}(1-\gamma)^{q-1} d \gamma \\
%& = \frac{1}{\mathrm{~B}(p, q)} \frac{1}{\sqrt{2 \pi \sigma_{\theta_S}^2}} \frac{\Gamma(p+1 / 2) \Gamma(q)}{\Gamma(p + q + 1/2)} \mathrm{M}\left(\frac{1}{2}+ p, \frac{1}{2}+ p+q,-\frac{\left(\hat{\theta}_S-\theta_T\right)^2}{2 \sigma_{\theta_S}^2}\right) \\
& \propto \mathrm{M}\left(\frac{1}{2}+ p, \frac{1}{2}+ p+q,-\frac{\left(\hat{\theta}_S-\theta_T\right)^2}{2 \sigma_{\theta_S}^2}\right),
\end{aligned}
\end{equation}
where $\mathrm{M}(a, b, z)=1 /(\Gamma(a) \Gamma(b-a)) \int_0^1 e^{z t} t^{a-1}(1-t)^{b-a-1} d t$ is Kummer's confluent hypergeometric function,  which is implemented in standard numerical mathematics libraries (note that the term $\Gamma(p + q + 1/2)$ in the numerator is omitted in \textcite{gravestock_adaptive_2017}) . 

Combining the joint prior $\pi\left(\theta_T, \gamma \mid \mathbf{D}_S\right)$ with the likelihood of the target study data produces a joint posterior for $\theta_T$ and $\gamma$, that is,
\begin{equation}
\begin{aligned}
\pi\left(\theta_T, \gamma \mid \mathbf{D}_T, \mathbf{D}_S\right) &= \frac{\mathcal{L}(\mathbf{D}_T \mid \theta_T) \pi\left(\theta_T, \gamma \mid \mathbf{D}_S\right)}{\int_0^1 \int_{-\infty}^{\infty} \mathcal{L}\left(\mathbf{D}_T \mid \theta_T^{\prime}\right) \pi\left(\theta_T^{\prime}, \gamma^{\prime} \mid \mathbf{D}_S\right) d \theta_T^{\prime} d \gamma^{\prime}} \\
&=\frac{\mathcal{N}\left(\hat{\theta}_T \mid \theta_T, \sigma_{\theta_T}^2\right) \mathcal{N}\left(\theta_T \mid \hat{\theta}_S, \sigma_{\theta_S}^2 / \gamma\right) \operatorname{Be}(\gamma \mid p, q)}{\int_0^1 \mathcal{N}\left(\hat{\theta}_T \mid \hat{\theta}_S, \sigma_{\theta_T}^2+\sigma_{\theta_S}^2 / \gamma^{\prime}\right) \operatorname{Be}\left(\gamma^{\prime} \mid p, q\right) d \gamma^{\prime}},
\end{aligned}
\end{equation}

from which a marginal posterior for $\gamma$ can be obtained by integrating out $\theta_T$, that is,
\begin{equation}
    \begin{aligned}
        \pi\left(\gamma \mid \mathbf{D}_T, \mathbf{D}_S\right) &=\int_{-\infty}^{+\infty} \pi\left(\theta_T, \gamma \mid \mathbf{D}_T, \mathbf{D}_S\right) d \theta_T \\ 
&= \frac{\mathcal{N}\left(\hat{\theta}_T \mid \hat{\theta}_S, \sigma_{\theta_T}^2+\sigma_{\theta_S}^2 / \gamma\right) \operatorname{Be}(\gamma \mid p, q)}{\int_0^1 \mathcal{N}\left(\hat{\theta}_T \mid \hat{\theta}_S, \sigma_{\theta_T}^2+\sigma_{\theta_S}^2 / \gamma^{\prime}\right) \operatorname{Be}\left(\gamma^{\prime} \mid p, q\right) d \gamma^{\prime}} \\
&\propto \mathcal{N}\left(\hat{\theta}_T \mid \hat{\theta}_S, \sigma_{\theta_T}^2+\sigma_{\theta_S}^2 / \gamma\right) \operatorname{Be}(\gamma \mid p, q).
    \end{aligned}
\end{equation}

The posterior distribution of the power parameter can therefore be approximated using numerical integration.

Moreover, \textcite{gravestock_adaptive_2017} show that: 
\begin{equation}
\begin{aligned}
\pi\left(\theta_T\mid \mathbf{D}_T, \mathbf{D}_S\right) &=  C(\gamma)\int_0^1\mathcal{N}\left(\hat{\theta}_T \mid \theta_T, \sigma_{\theta_T}^2\right) \mathcal{N}\left(\theta_T \mid \hat{\theta}_S, \sigma_{\theta_S}^2 / \gamma\right) \operatorname{Be}(\gamma \mid p, q) d\gamma\\
%& =C(\gamma)\mathcal{N}\left(\hat{\theta}_T \mid \theta_T, \sigma_{\theta_T}^2\right)  \int_0^1 \mathcal{N}\left(\theta_T \mid \hat{\theta}_S, \sigma_{\theta_S}^2 / \gamma\right) \operatorname{Be}(\gamma \mid p, q) d\gamma\\
%& =C(\gamma)\mathcal{N}\left(\hat{\theta}_T\mid \theta_T, \sigma_{\theta_T}^2\right) \pi\left(\theta_T\mid \mathbf{D}_S\right) \\
&\propto \operatorname{exp}\left(- \frac{( \hat{\theta}_T-  \theta_T)^2}{2\sigma_{\theta_T}^2} \right) \mathrm{M}\left(\frac{1}{2}+ p, \frac{1}{2}+ p+q,-\frac{\left(\hat{\theta}_S-\theta_T\right)^2}{2 \sigma_{\theta_S}^2}\right).
\end{aligned}
\end{equation}

When implementing this model, we took inspiration from the code in \textcite{pawel_normalized_2023}, which relies on numerical integration instead of the full analytical expression that includes the confluent hypergeometric function. We noticed that computing the posterior using the full analytical expression was faster than using numerical integration. However, when using adaptive quadrature to compute the mean and variance of the distribution, using numerical integration to obtain the posterior density led to a much faster computation compared to using the full analytical expression, yet with similar accuracy.  Therefore, we instead relied on numerical integration to compute the posterior distribution.
To better interpret this prior, we reparameterize it as  $\gamma \sim Beta(\xi_\gamma/\omega_\gamma,(1-\xi_\gamma)/\omega_\gamma)$, where $\mathbb{E}[\gamma] = \xi_\gamma$ and $\mathbb{V}[\gamma] = \sigma_\gamma^2 = \frac{\omega_\gamma \xi_\gamma (1-\xi_\gamma)}{1+\omega_\gamma}$.
We used $\xi_\gamma = 0.5$ , and vary $\omega_\gamma$ so that the standard deviation of the Beta prior ranges from 0 to 0.50. We have: $\omega_\gamma = \frac{\sigma^2_\gamma}{\xi_\gamma(1-\xi_\gamma) - \sigma_\gamma^2} $.

\subsection{Estimation of posterior distributions}
\paragraph{Markov Chain Monte Carlo}

In the Bayesian framework, all information about the target treatment effect is summarized in the posterior distribution 
$p(\theta_T\mid\mathbf{D}_S = d_S,\mathbf{D}_T= d_T)$.  
In many cases, however, this posterior distribution cannot be computed analytically, but several methods exist to approximate it. In the simulation study, when possible, we relied on numerical integration to compute the posterior distribution, or on Markov chain Monte Carlo (MCMC) simulation techniques to draw approximate samples from the posterior distribution. 
These samples then allowed us to estimate quantities of interest, such as the posterior mean, median, and other quantiles.

We used the probabilistic programming language Stan for running MCMC.
Given that all parameters in the models are continuous, we used the default sampler in Stan, the No-U-Turn Sampler (NUTS, \textcite{hoffman_no-u-turn_2011}), an advanced and highly efficient MCMC sampling algorithm. Unless required because of convergence issues or strong autocorrelation, we used Stan's default parameters for NUTS . 

\paragraph{Number of chains} Using multiple chains with random initial values makes the convergence diagnostic more accurate (see Section \ref{sec:convergence_diagnostics}), and is safer in situations where the posterior distribution is multi-modal. That is, it mitigates the risk of having the chain circumscribed around a mode, and potentially allows identifying multimodality. This can lead to a better approximation of the posterior, even if between-chain mixing is not achieved.  
As a consequence, we used 4 chains. 

\paragraph{Initial values} Treatment effect parameters and hyperparameters were initialized by taking samples from their respective prior (or hyperprior) distributions. 

%\paragraph{Thinning} In the past, it was common to "thin" MCMC simulations, discarding all but every k$^{th}$ sampled values to reduce autocorrelation while reducing memory burden. However, in practice, it is now considered better to keep autocorrelated samples than to remove them, and samplers such as NUTS tend to have very low auto-correlation. Therefore, we did not use thinning.

\paragraph{MCMC Effective Sample Size}

 The MCMC effective sample size (MCMC ESS) represents the number of independent samples from the posterior distribution that provide the same amount of information as the correlated draws generated by MCMC. In other words, it quantifies the efficiency of the MCMC algorithm in exploring the posterior distribution. An MCMC ESS is estimated for each parameter. Aiming for a sufficiently large MCMC ESS is crucial for reliable estimation. 

Moreover, a crucial quantity estimated from MCMC draws is $\operatorname{Pr}(\theta_T  \notin\Theta_0)$. Indeed, it is concluded that the treatment is effective if $\operatorname{Pr}(\theta_T  \notin\Theta_0)  > \eta$, with $\eta = 0.975$. Therefore, we need to ensure that we get a precise estimate of the 0.975th sample quantile. 

The reasoning used to determine the standard deviation of sample quantiles is given in appendix \ref{appendix}, allowing us to conclude that if we want the 0.975th sample quantile to be estimated with the same precision as the median, we would need $1/0.47 = 2.14$  times more samples. 

Based on these considerations, we ensured that the MCMC effective sample size for the target trial treatment effect parameter $\theta_T$ is at least 10,000 and adapt the chains’ length consequently. Assuming a posterior that is a standard normal distribution, this would correspond to a standard error on the median estimate of 0.0125, and a standard error on the 0.975th sample quantile estimate of 0.0267. Concretely, with $N_C = 4$ chains of length $L$, for each simulated data replicate, we computed the MCMC ESS for the target treatment effect $\epsilon_{\theta_T}$. We then adjusted the chain length so that $L \leftarrow  1.1 \times L \times \epsilon_{\theta_T}/\epsilon$, where $\epsilon$ is the target MCMC ESS of 10,000, and repeated the iteration until sufficient MCMC, that is, until $\epsilon_{\theta_T}>\epsilon$. To avoid an explosion of chains length, we capped $L$ to 10,000. By contrast, for speed gains, we reduced chain lengths when $\epsilon_{\theta_T}> 1.1 \times \epsilon$, applying  $L \leftarrow  1.1 \times L \times \epsilon_{\theta_T}/\epsilon$, and proceeded to the next data replicates.

\paragraph{Convergence diagnostics}
\label{sec:convergence_diagnostics}

By definition, a Markov chain generates samples from the target distribution only after it has converged to equilibrium. In theory, convergence is only guaranteed asymptotically, therefore, in practice, diagnostics must be applied to monitor convergence for the finite number of draws actually available.
Therefore, at the model development stage, when using MCMC, Markov Chains visual inspection was performed using tools such as trace plots and autocorrelation plots to verify that the MCMC chains have reached a stationary distribution.
To automate the MCMC convergence diagnostic for each replicate, we used the Gelman and Rubin (1992) potential scale reduction statistic $\widehat{R}$ to monitor convergence. $\widehat{R}$  measures the ratio of the average variance of samples within each chain to the variance of the pooled samples across chains. If all chains are at equilibrium, these will be the same and $\widehat{R}$  will be one, and greater otherwise. Gelman and Rubin’s recommendation is that the independent Markov chains be initialized with diffuse starting values for the parameters and sampled until all values for $\widehat{R}$ are below 1.1. We also monitored the number of transitions ending with a divergence.

%Before Stan calculating the potential-scale-reduction statistic $\widehat{R}$, each chain is split into two halves. This provides an additional means to detect non-stationarity in the individual chains. If one chain involves gradually increasing values and one involves gradually decreasing values, they have not mixed well, but they can have $\widehat{R}$ values near unity. In this case, splitting each chain into two parts leads to $\widehat{R}$ values (split-$\widehat{R}$ ) substantially greater than 1 because the first half of each chain has not mixed with the second half. 

Execution of the code does not stop in case of issues with MCMC inference; rather, a warning is stored in the results table so that the pipeline is not interrupted. In case of convergence issues, we adapted the MCMC algorithm by increasing the acceptance probability of the sampler, the tuning period, and reparameterizing the distribution.
These convergence diagnoses also allowed us to determine if some models have particular behaviors that need specific handling.

\subsubsection{Standard deviation of the sample quantiles}

To determine the standard deviation of sample quantiles, we follow the following reasoning: let $Y$ be a continuous random variable with probability density function $f$, for which we have a sample of size $n$.
We are interested in determining the distribution of the sample median and 0.975th quantile, denoted $X_q$ (with  $q_1 = 0.5$ and $q_2 = 0.975$ respectively). 
We adapt the reasoning developed by Dr William A. Huber in  \url{https://stats.stackexchange.com/a/86804/919}.

Let's denote $G_q$ the c.d.f. of $Beta(\alpha, \beta)$, with $\alpha = qn+1$ and $\beta = (1-q)n+1$. 
Then, the c.d.f. of $X_q$ in $x$ is $G_q(F(x))$, so that the p.d.f. of $X_q$ is:
$\frac{\partial G_q\circ  F}{\partial x}(x) = g_q(F(x))f(x)$.

So the p.d.f. of the sample quantile is  $g_q(F(x))f(x)$. 

Now we are interested in approximating the variance of this distribution.

By denoting $\mu_q = F^{-1}(q)$, we have, for sufficiently well-behaved $F$:

\begin{equation}
\begin{aligned}
     F(x) &= F(\mu_q + (x-\mu_q)) \\
     &\approx F(\mu_q) + F'(\mu_q)(x-\mu_q) \\
     &\approx q + f(\mu_q)(x-\mu_q) 
\end{aligned}
\end{equation} 

So, assuming $f$  is continuous near $\mu_q$, the p.d.f. of $X_q$ is approximately : $g_q(q + f(\mu_q)(x-\mu_q))f(\mu_q)$. This is essentially a shift of the location and scale of the Beta distribution. The variance of $Beta(\alpha, \beta)$ is :$$\frac{\alpha \beta}{(\alpha + \beta)^2(\alpha + \beta + 1)},$$
so that the variance of the sample quantile is approximately:
$$\frac{\alpha \beta}{(\alpha + \beta)^2(\alpha + \beta + 1)f(F^{-1}(q))^2},$$

So, for large $n$, this variance can be approximated as : $\frac{q(1-q)}{nf(F^{-1}(q))^2}$.
So for two different quantiles $q_1$ and $q_2$, the ratio of standard error on the sample quantile is approximately : 
$$\sqrt{\frac{q_1(1-q_1)}{q_2(1-q_2)}}\frac{f(F^{-1}(q_2))}{f(F^{-1}(q_1))}$$

For the standard normal distribution, with $q_1 = 0.5$ and $q_2 = 0.975$, this gives a ratio of 0.47.

\newpage
\section{Supplementary tables}

\subfile{Tables_protocol/Sample_sizes_table.tex}
\subfile{Tables_protocol/drift_ranges_table.tex}

\subfile{Tables_protocol/study_protocol_table_with_ranges.tex}

%\subfile{Tables_protocol/prior_heterogeneity.tex}
  
\subfile{Tables_protocol/Bayesian_OCs.tex}

%\subfile{Tables_protocol/Approximations.tex}

\subfile{Tables_protocol/RCTs_selection_table.tex}

\subfile{Tables_protocol/table_configuration.tex}
\subfile{Tables_protocol/table_configuration_intensive.tex}

\clearpage
\newpage

\section{Supplementary figures}

%All figures are available as a supplementary zip file. Below are the figures referenced in the main text.

\subfile{Figures_protocol/graphical_model_binomial_likelihood.tex} 
 
\subfile{Figures_protocol/simulation_pipeline_v4}

\clearpage
\subsection{Probability of study success as a function of the drift in treatment effect}

\begin{figure}[htbp]
    \centering
    \includegraphics[width=1\linewidth]{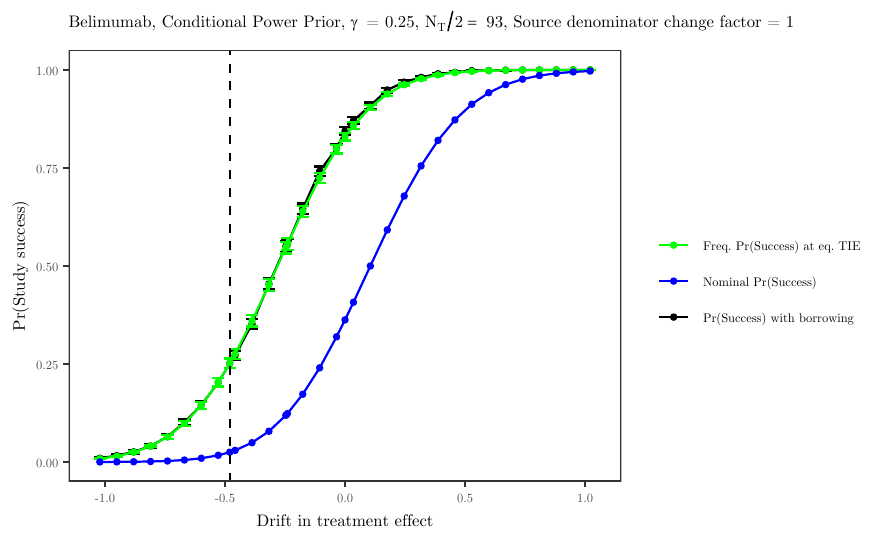}
    \caption{Probability of success of the Conditional Power Prior with $\gamma = 0.25$ as a function of the drift in treatment effect (black) in the Belimumab case study at a sample size per arm of 93, without change introduced in the denominator of the source study summary measure. The probability of success of the t-test at a nominal type 1 error rate of $0.025$ as a function of drift is displayed in blue. The probability of success of the t-test at a type 1 error rate equal to the Conditional PP type 1 error rate is displayed in green.
    Borrowing of external data that favors the null hypothesis also implies that the probability of success of the borrowing method is always larger, in the alternative hypothesis space, than the probability of success of the frequentist method at the nominal type 1 error rate of 0.025. The power curves at equivalent type 1 error rate are identical.
$\theta_T = \theta_0$ is indicated by a dashed line. Error bars correspond to the 95\% CI of the metric.}
    \label{fig:power_equivalent_tie}
\end{figure}

\begin{figure}[htbp]
    \centering
    \includegraphics[width=1\linewidth]{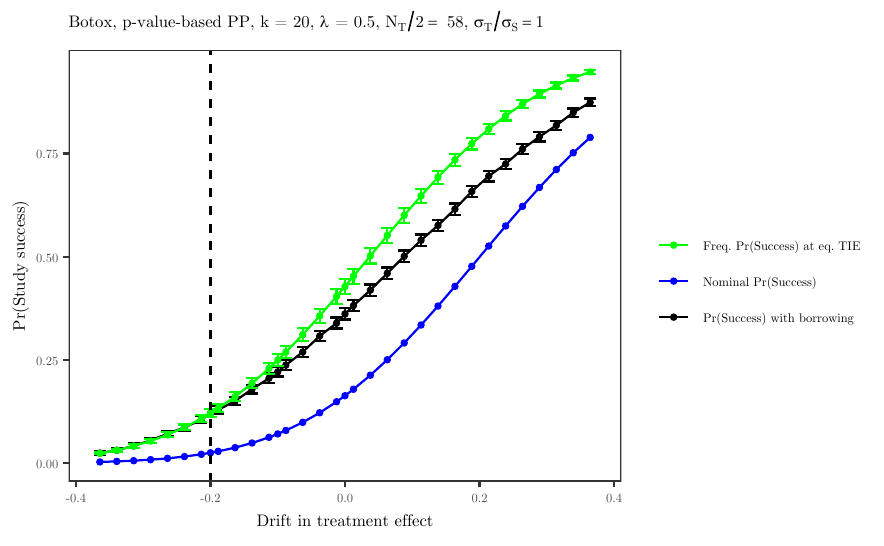}
    \caption{Probability of success of the p-value-based Power Prior with parameters $k= 20$ and $\lambda = 20$ as a function of the drift in treatment effect (black) in the Botox case study at a sample size per arm of 58, with a sampling standard deviation equal between the source and target study. The probability of success of the t-test at a nominal type 1 error rate of $0.025$ as a function of drift is displayed in blue. The probability of success of the t-test at a type 1 error rate equal to the p-value based PP type 1 error rate is displayed in green. $\theta_T = \theta_0$ is indicated by a dashed line. In this example, the power of the p-value based power prior is lower than the power of the frequentist t-test at equivalent type 1 error rate in the whole alternative hypothesis space. Error bars correspond to the 95\% CI of the probability of success.}
    \label{fig:power_loss}
\end{figure}

\clearpage

\subsection{Supplementary figures for the Botox case study (continuous endpoint).}

\begin{figure}[htbp]
    \centering
    \includegraphics[width=1\linewidth]{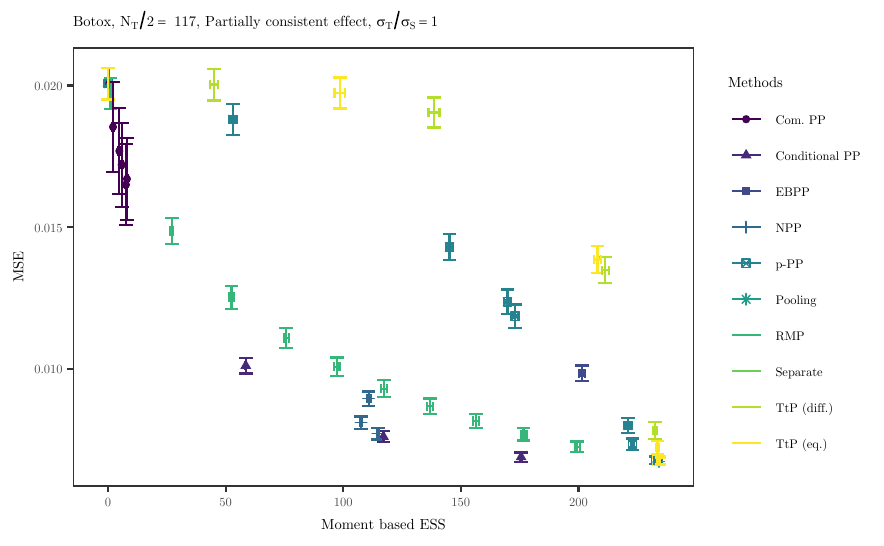}
    \caption{MSE as a function of the mean moment-based ESS in the Botox case study with a sample size per arm of 117. Error bars correspond to the 95\% CI of the MSE. TtP (diff.) : test-then-pool with a test for difference. 
TtP (eq.) : test-then-pool with a test for equivalence. p-PP : p-value-based Power Prior. 
EBPP: Empirical Bayes Power Prior.
RMP : Robust Mixture Prior. 
Conditional PP : Conditional Power Prior.  
NPP : Normalized Power Prior 
Com. PP : Commensurate Power Prior. 
Separate : separate analysis of the target trial data.}
    \label{fig:botox_mse_vs_ess_moment_sample_size=117_treatment_effect=partially_consistent}
\end{figure}

\begin{figure}[h!]
\centering
\includegraphics[width=1\linewidth]{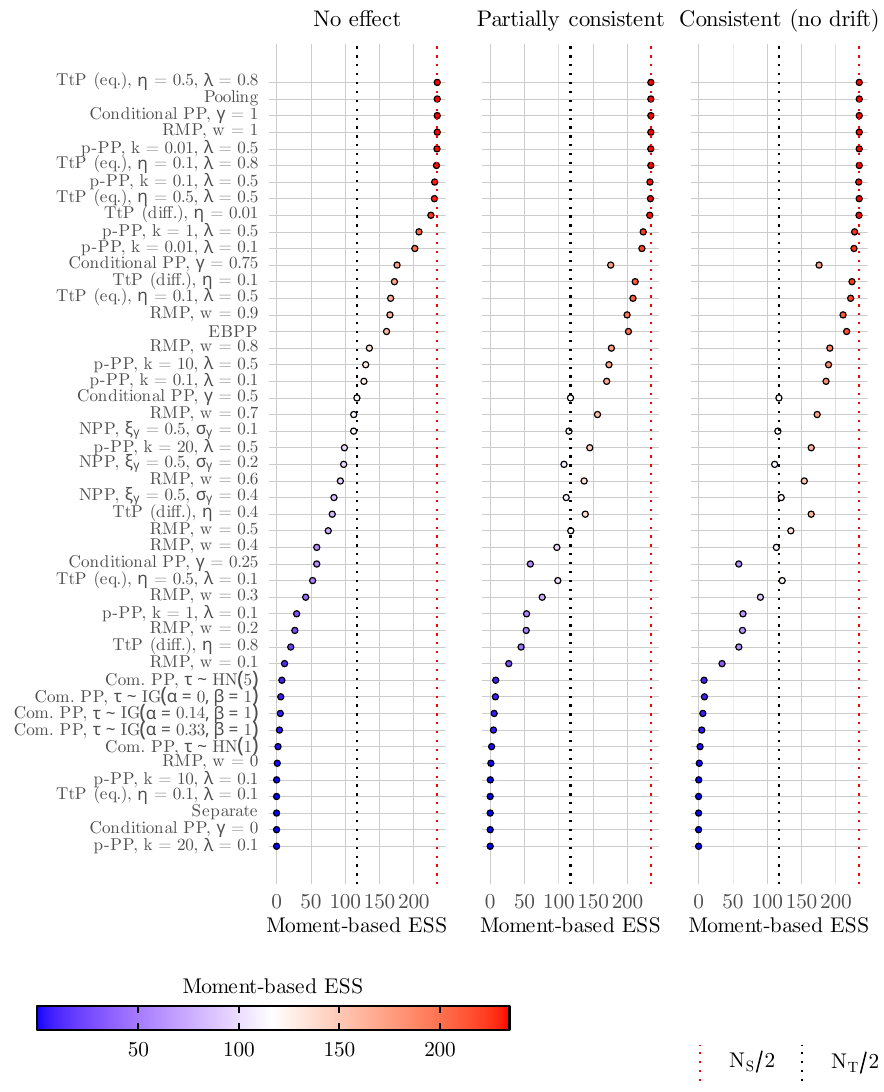}
\caption{Moment-based ESS across methods and for the three main treatment effects considered in the Botox case study with $N_T/2 = 117$. The red dashed line corresponds to an ESS equal to the source study sample size per arm, and the black dashed line corresponds to the target study sample size per arm. The dashed vertical line indicates the nominal TIE. TtP (diff/eq) : test-then-pool with a test for difference/equivalence ($\eta$: significance level of the test. $\lambda$: equivalence margin ). Conditional PP : Conditional Power Prior ($\gamma$: power parameter). p-PP : p-value-based PP ($k$: shape parameter, $\lambda$: equivalence margin). EBPP: Empirical Bayes PP.
RMP : Robust Mixture Prior ($w$: weight of the informative prior component). NPP : Normalized PP ($\xi_\gamma$ and $\sigma_\gamma$ are respectively the mean and standard deviation of the Beta prior on the power parameter $\gamma$). Com. PP : Commensurate PP ($\tau$: heterogeneity parameter). Separate : separate analysis of the target trial data alone.}
\label{fig:botox_ess_moment_forest_plot_117}
\end{figure}

\begin{figure}[htbp]
    \centering
    \includegraphics[width=1\linewidth]{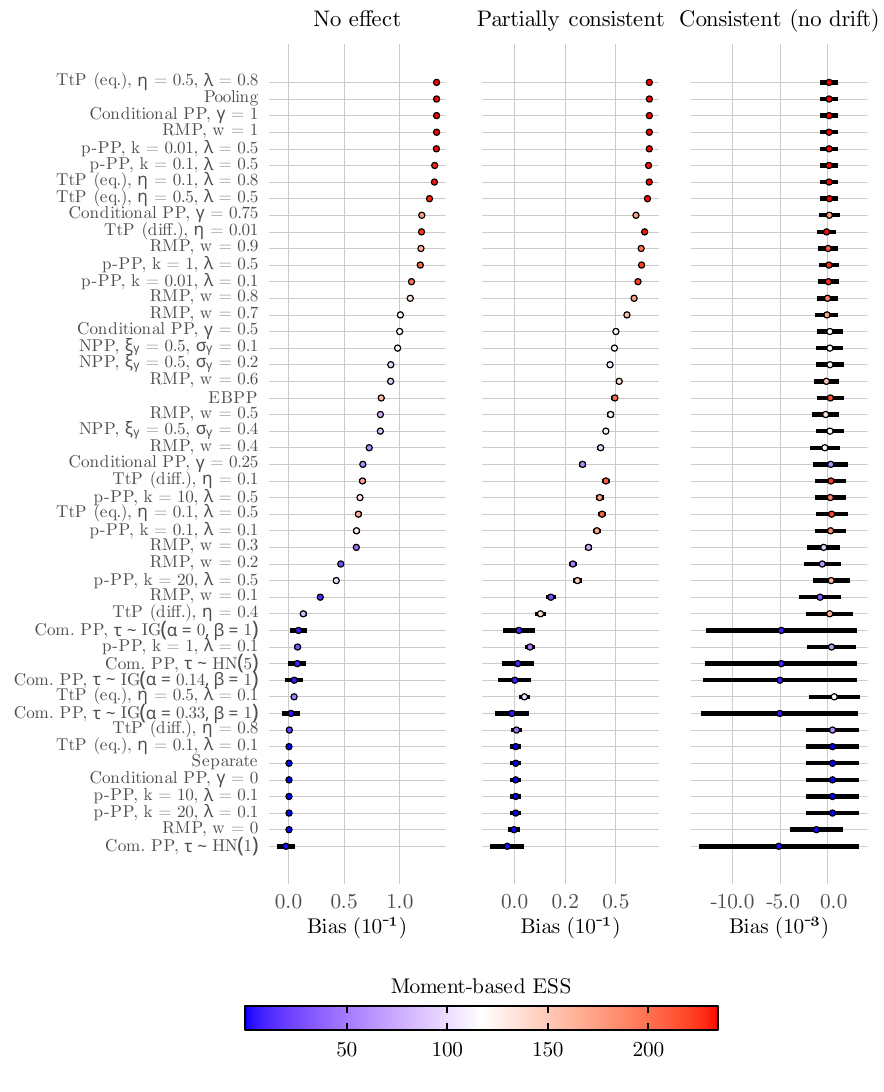}
    \caption{Bias and associated 95\% CI, for the three main treatment effects considered, in the Botox case study ($N_T=117$)). TtP (diff/eq) : test-then-pool with a test for difference/equivalence ($\eta$: significance level of the test. $\lambda$: equivalence margin ). Conditional PP : Conditional Power Prior ($\gamma$: power parameter). p-PP : p-value-based PP ($k$: shape parameter, $\lambda$: equivalence margin). EBPP: Empirical Bayes PP.
RMP : Robust Mixture Prior ($w$: weight of the informative prior component). NPP : Normalized PP ($\xi_\gamma$ and $\sigma_\gamma$ are respectively the mean and standard deviation of the Beta prior on the power parameter $\gamma$). Com. PP : Commensurate PP ($\tau$: heterogeneity parameter). Separate : separate analysis of the target trial data alone.}
    \label{fig:botox_bias_forest_plot_target_sample_size_per_arm_117}
\end{figure}

\begin{figure}[htbp]
    \centering
    \includegraphics[width=1\linewidth]{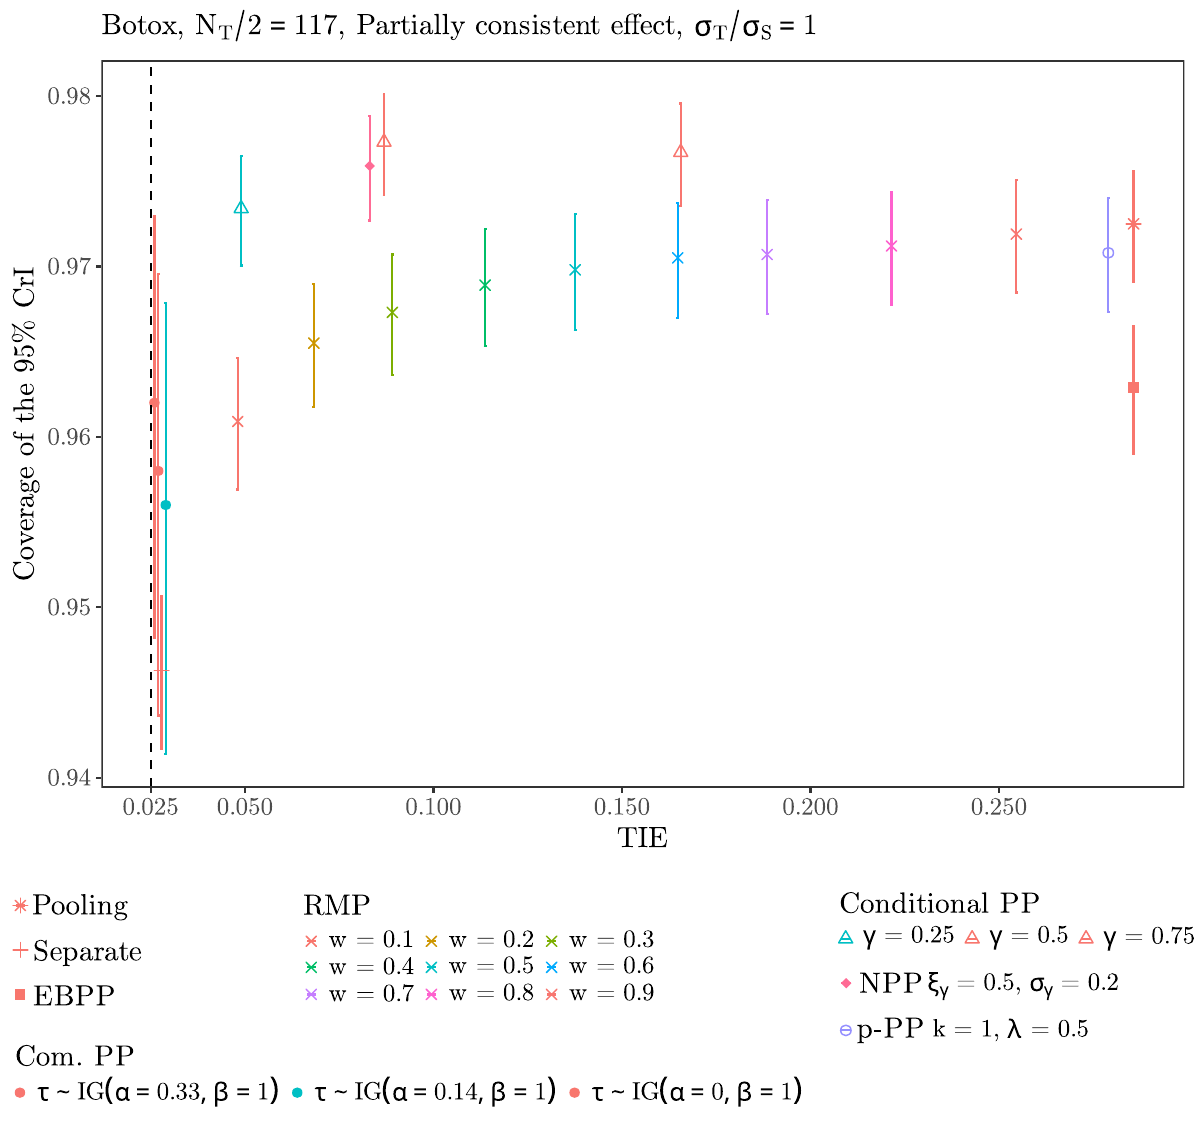}
    \caption{Coverage of the 95\% Confidence Interval as a function of type 1 error rate in the Botox case study with a sample size per arm of $117$, across all the methods and parameters, without treatment effect. The target to source standard deviation ratio is $1$. Error bars correspond to the 95\% CI of the Coverage and type 1 error rate. Dashed vertical line represents the nominal type 1 error rate of $0.025$.
    TtP (diff/eq) : test-then-pool with a test for difference/equivalence ($\eta$: significance level of the test. $\lambda$: equivalence margin ). Conditional PP : Conditional Power Prior ($\gamma$: power parameter). p-PP : p-value-based PP ($k$: shape parameter, $\lambda$: equivalence margin). EBPP: Empirical Bayes PP.
RMP : Robust Mixture Prior ($w$: weight of the informative prior component). NPP : Normalized PP ($\xi_\gamma$ and $\sigma_\gamma$ are respectively the mean and standard deviation of the Beta prior on the power parameter $\gamma$). Com. PP : Commensurate PP ($\tau$: heterogeneity parameter). Separate : separate analysis of the target trial data alone.}
    \label{fig:botox_coverage_vs_tie_sample_size=117_treatment_effect=partially_consistent}
\end{figure}

\begin{figure}
    \centering
    \includegraphics[width=1\linewidth]{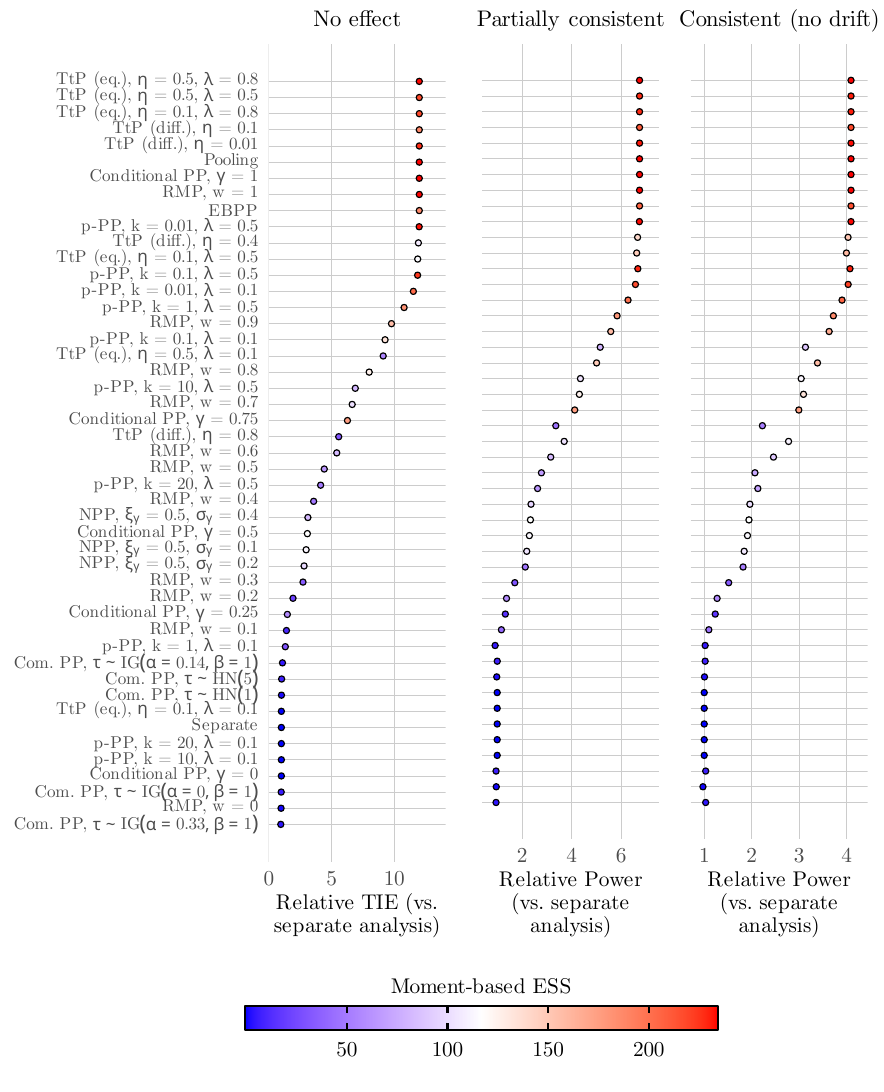}
    \caption{TIE and power relative to a separate analysis for the three main treatment effects considered, in the Botox case study ($N_T/2=58$).
    TtP (diff/eq) : test-then-pool with a test for difference/equivalence ($\eta$: significance level of the test. $\lambda$: equivalence margin ). Conditional PP : Conditional Power Prior ($\gamma$: power parameter). p-PP : p-value-based PP ($k$: shape parameter, $\lambda$: equivalence margin). EBPP: Empirical Bayes PP.
RMP : Robust Mixture Prior ($w$: weight of the informative prior component). NPP : Normalized PP ($\xi_\gamma$ and $\sigma_\gamma$ are respectively the mean and standard deviation of the Beta prior on the power parameter $\gamma$). Com. PP : Commensurate PP ($\tau$: heterogeneity parameter). Separate : separate analysis of the target trial data alone.
}
    \label{fig:botox_relative_success_proba_forest_plot_target_sample_size_per_arm_58}
\end{figure}

\clearpage
\subsection{Supplementary figures for the Dapagliflozin case study (continuous endpoint).}

\begin{figure}[htbp]
    \centering
    \includegraphics[width=1\linewidth]{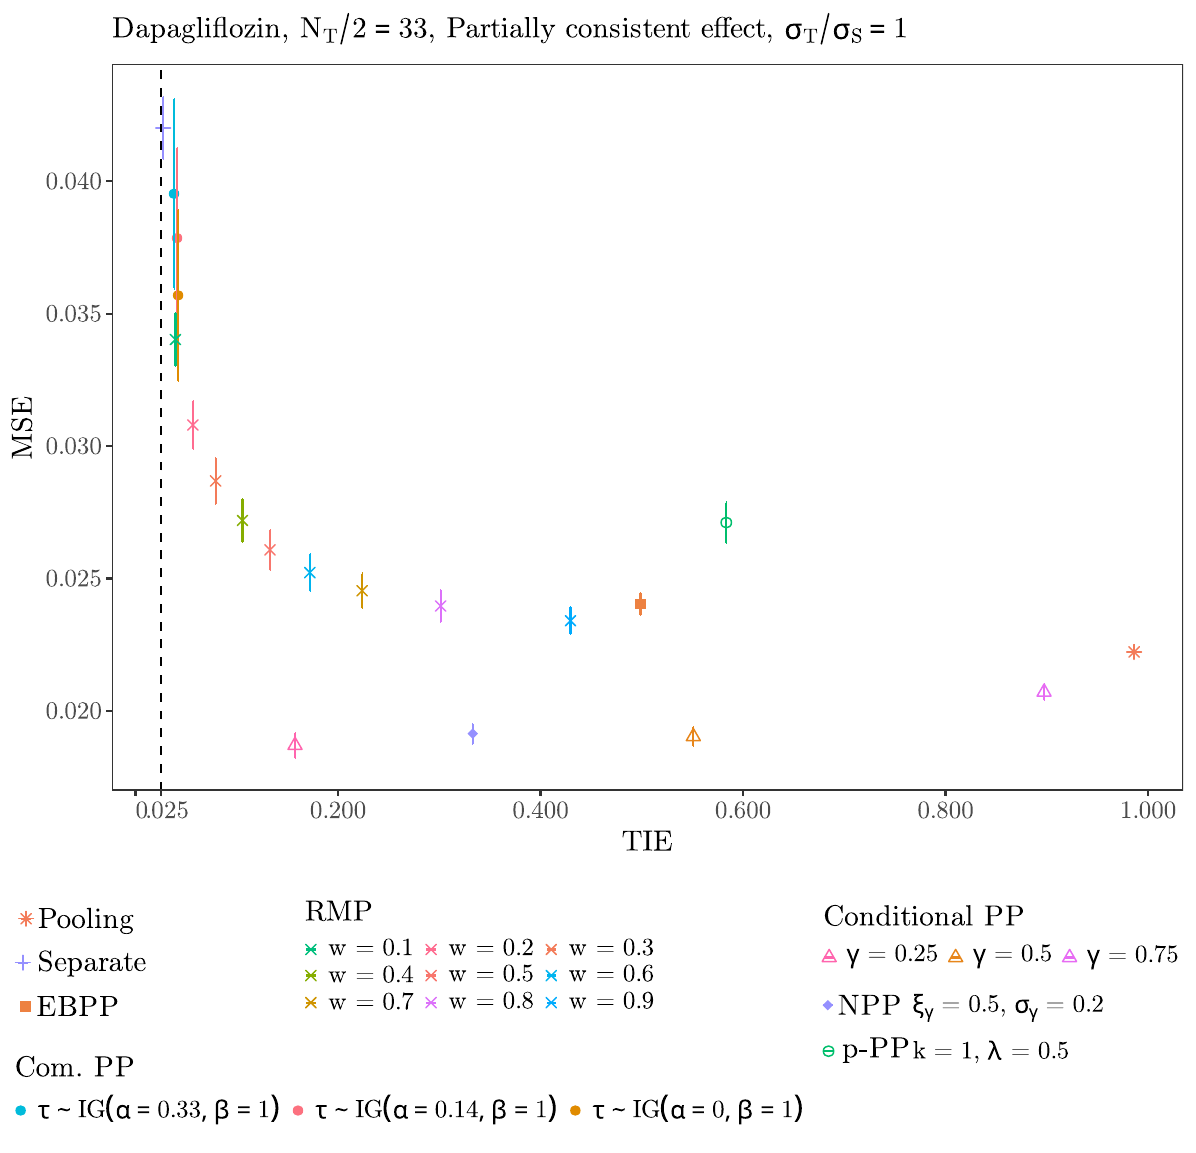}
    \caption{MSE as a function of type 1 error rate in the Dapagliflozin case study with a sample size per arm of $33$, across all the methods and parameters, with a partially consistent treatment effect. Error bars correspond to the 95\% CI. Dashed vertical line represents the nominal type 1 error rate of $0.025$.
    TtP (diff/eq) : test-then-pool with a test for difference/equivalence ($\eta$: significance level of the test. $\lambda$: equivalence margin ). Conditional PP : Conditional Power Prior ($\gamma$: power parameter). p-PP : p-value-based PP ($k$: shape parameter, $\lambda$: equivalence margin). EBPP: Empirical Bayes PP.
RMP : Robust Mixture Prior ($w$: weight of the informative prior component). NPP : Normalized PP ($\xi_\gamma$ and $\sigma_\gamma$ are respectively the mean and standard deviation of the Beta prior on the power parameter $\gamma$). Com. PP : Commensurate PP ($\tau$: heterogeneity parameter). Separate : separate analysis of the target trial data alone.
}
\label{fig:dapagliflozin_mse_vs_tie_sample_size=33_treatment_effect=partially_consistent}
\end{figure}
 
 \begin{figure}[htbp]
\centering
\includegraphics[width=1\linewidth]{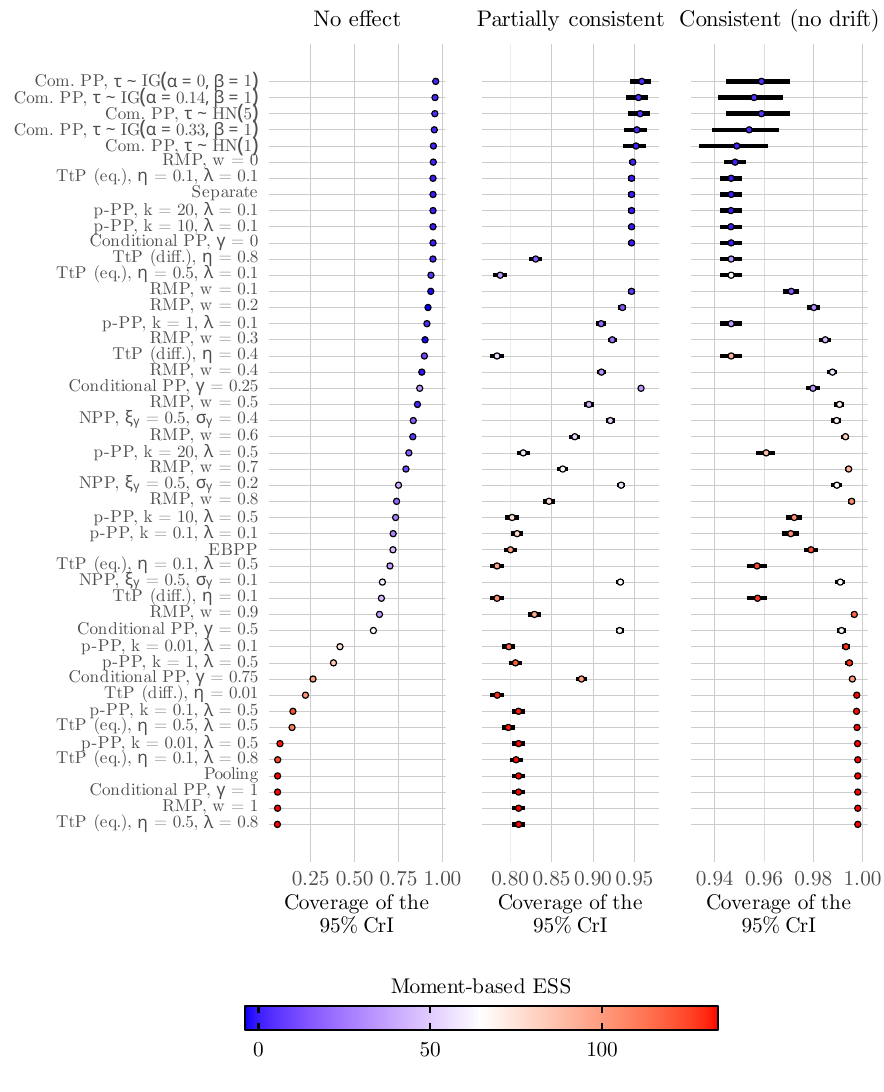}
\caption{Coverage probability of the 95\% CrI for the three main treatment effect values considered in the Dapagliflozin case study ($N_T/2=66$). Error bars correspond to the 95\% CI on the coverage probability.
TtP (diff/eq) : test-then-pool with a test for difference/equivalence ($\eta$: significance level of the test. $\lambda$: equivalence margin ). Conditional PP : Conditional Power Prior ($\gamma$: power parameter). p-PP : p-value-based PP ($k$: shape parameter, $\lambda$: equivalence margin). EBPP: Empirical Bayes PP.
RMP : Robust Mixture Prior ($w$: weight of the informative prior component). NPP : Normalized PP ($\xi_\gamma$ and $\sigma_\gamma$ are respectively the mean and standard deviation of the Beta prior on the power parameter $\gamma$). Com. PP : Commensurate PP ($\tau$: heterogeneity parameter). Separate : separate analysis of the target trial data alone.
}
\label{fig:dapagliflozin_coverage_forest_plot_target_sample_size_per_arm_66}
\end{figure}

\begin{figure}[htbp]
\centering
\includegraphics[width=1\linewidth]{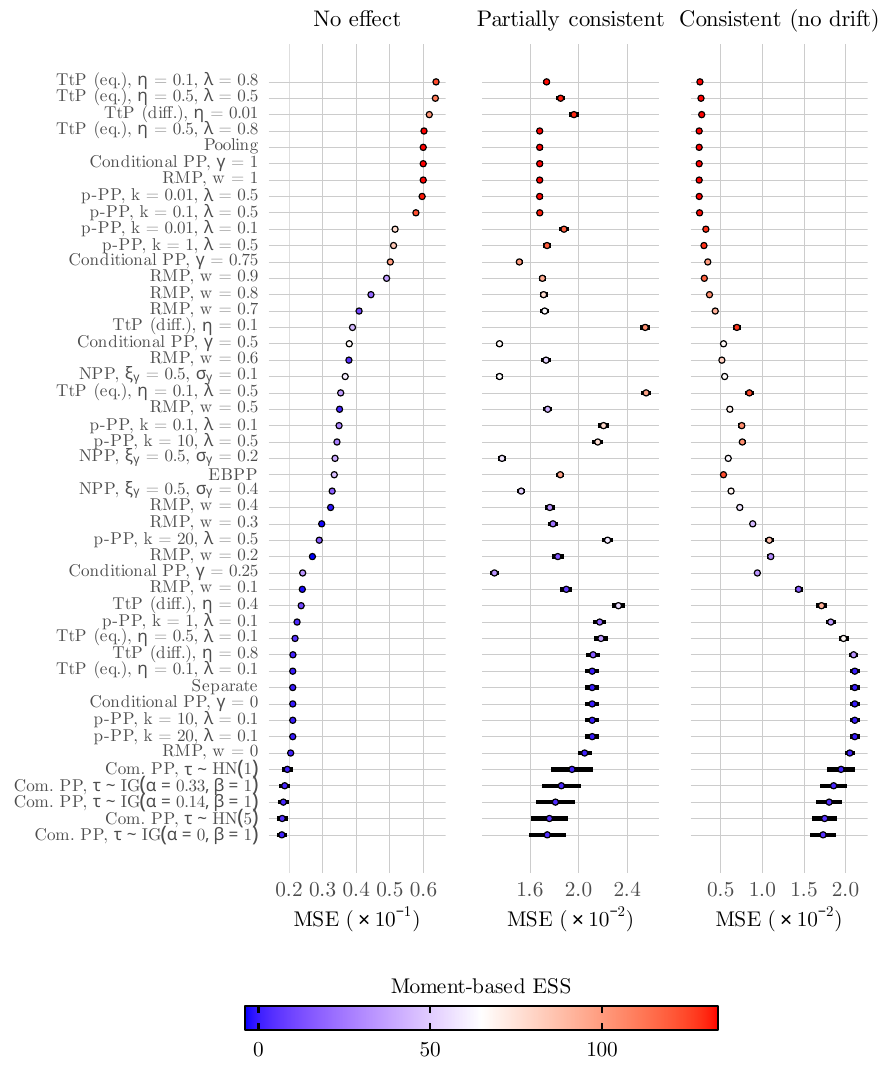}
\caption{MSE for the three main treatment effect values considered in the Dapagliflozin case study ($N_T/2=66$).  
TtP (diff/eq) : test-then-pool with a test for difference/equivalence ($\eta$: significance level of the test. $\lambda$: equivalence margin ). Conditional PP : Conditional Power Prior ($\gamma$: power parameter). p-PP : p-value-based PP ($k$: shape parameter, $\lambda$: equivalence margin). EBPP: Empirical Bayes PP.
RMP : Robust Mixture Prior ($w$: weight of the informative prior component). NPP : Normalized PP ($\xi_\gamma$ and $\sigma_\gamma$ are respectively the mean and standard deviation of the Beta prior on the power parameter $\gamma$). Com. PP : Commensurate PP ($\tau$: heterogeneity parameter). Separate : separate analysis of the target trial data alone.
}
\label{fig:dapagliflozin_mse_forest_plot_target_sample_size_per_arm_66}
\end{figure} 

\begin{figure}[htbp]
\centering
\includegraphics[width=1\linewidth]{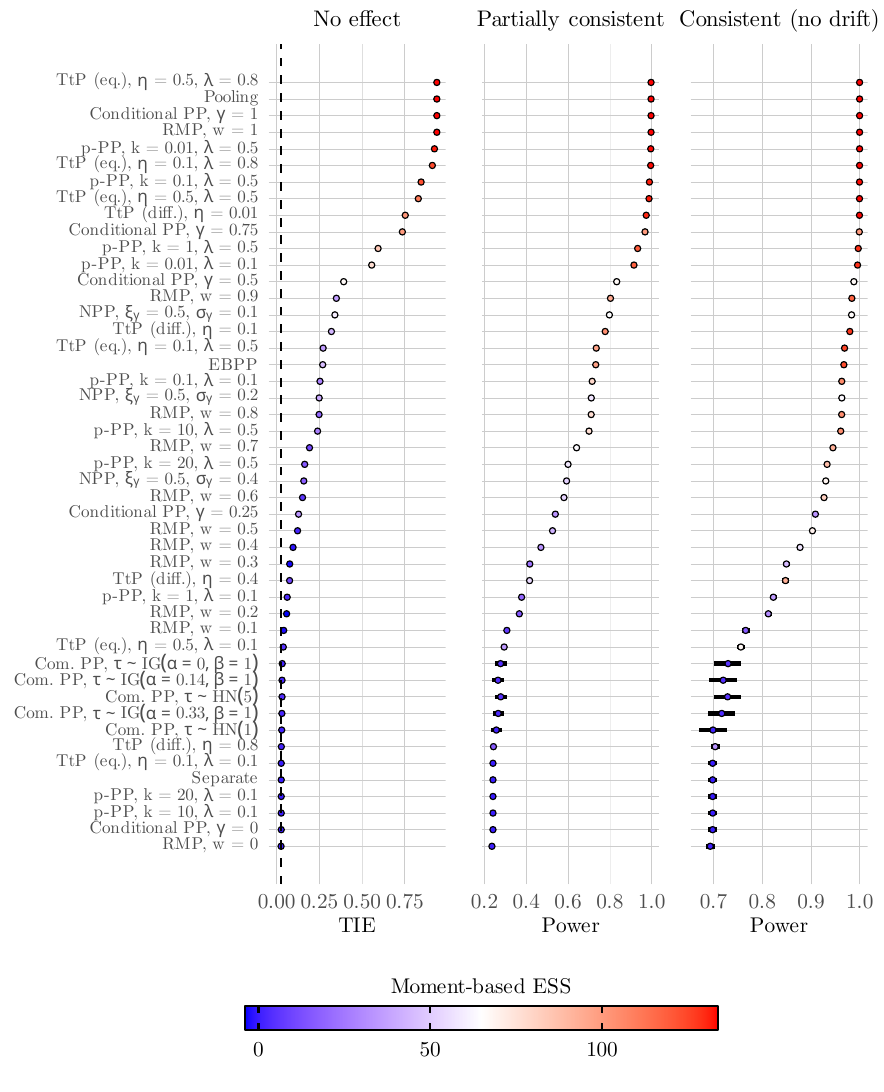}
\caption{Probability of study success for the three main treatment effect values considered in the Dapagliflozin case study ($N_T/2=66$).  
TtP (diff/eq) : test-then-pool with a test for difference/equivalence ($\eta$: significance level of the test. $\lambda$: equivalence margin ). Conditional PP : Conditional Power Prior ($\gamma$: power parameter). p-PP : p-value-based PP ($k$: shape parameter, $\lambda$: equivalence margin). EBPP: Empirical Bayes PP.
RMP : Robust Mixture Prior ($w$: weight of the informative prior component). NPP : Normalized PP ($\xi_\gamma$ and $\sigma_\gamma$ are respectively the mean and standard deviation of the Beta prior on the power parameter $\gamma$). Com. PP : Commensurate PP ($\tau$: heterogeneity parameter). Separate : separate analysis of the target trial data alone.
}
\label{fig:dapagliflozin_success_proba_forest_plot_target_sample_size_per_arm_66}
\end{figure} 

\begin{figure}[htbp]
\centering
\includegraphics[width=1\linewidth]{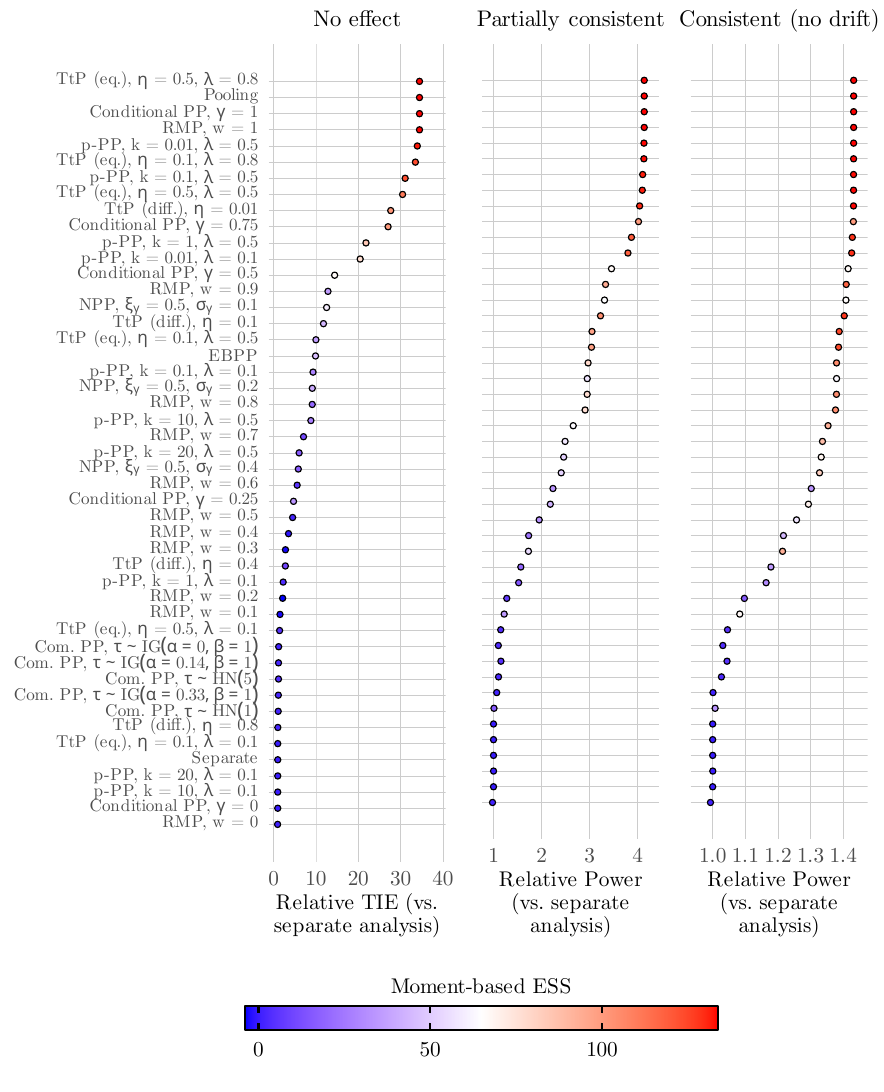}
\caption{Probability of study success of the 95\% CrI for the three main treatment effect values considered in the Dapagliflozin case study ($N_T/2=66$), relative to the probability of success for a separate analysis of the target study data.  
TtP (diff/eq) : test-then-pool with a test for difference/equivalence ($\eta$: significance level of the test. $\lambda$: equivalence margin ). Conditional PP : Conditional Power Prior ($\gamma$: power parameter). p-PP : p-value-based PP ($k$: shape parameter, $\lambda$: equivalence margin). EBPP: Empirical Bayes PP.
RMP : Robust Mixture Prior ($w$: weight of the informative prior component). NPP : Normalized PP ($\xi_\gamma$ and $\sigma_\gamma$ are respectively the mean and standard deviation of the Beta prior on the power parameter $\gamma$). Com. PP : Commensurate PP ($\tau$: heterogeneity parameter). Separate : separate analysis of the target trial data alone.
}
\label{fig:dapagliflozin_relative_success_proba_forest_plot_target_sample_size_per_arm_66}
\end{figure} 

\clearpage
\subsection{Supplementary figures for the Belimumab case study (binary endpoint with normal approximation).}

\begin{figure}[htbp]
    \centering
    \includegraphics[width=1\linewidth]{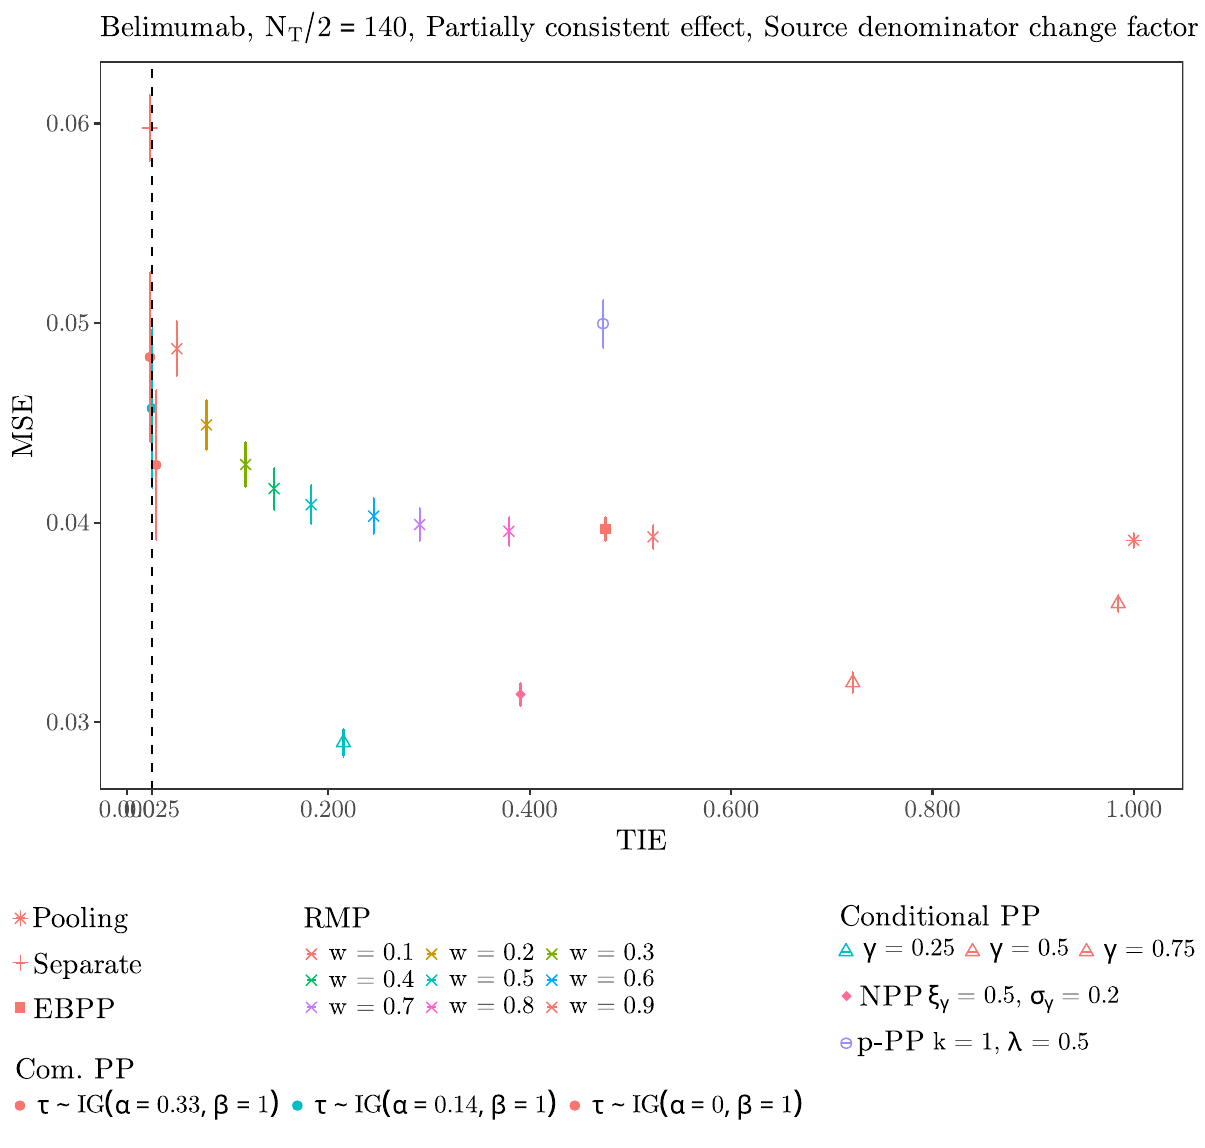}
    \caption{MSE as a function of type 1 error rate in the Belimumab case study with a sample size per arm of $140$, across all the methods and parameters, with a partially consistent treatment effect. Error bars correspond to the 95\% CI. Dashed vertical line represents the nominal type 1 error rate of $0.025$.
    TtP (diff/eq) : test-then-pool with a test for difference/equivalence ($\eta$: significance level of the test. $\lambda$: equivalence margin ). Conditional PP : Conditional Power Prior ($\gamma$: power parameter). p-PP : p-value-based PP ($k$: shape parameter, $\lambda$: equivalence margin). EBPP: Empirical Bayes PP.
RMP : Robust Mixture Prior ($w$: weight of the informative prior component). NPP : Normalized PP ($\xi_\gamma$ and $\sigma_\gamma$ are respectively the mean and standard deviation of the Beta prior on the power parameter $\gamma$). Com. PP : Commensurate PP ($\tau$: heterogeneity parameter). Separate : separate analysis of the target trial data alone.
}
    \label{fig:belimumab_mse_vs_tie_sample_size=140_treatment_effect=partially_consistent}
\end{figure}

\begin{figure}[htbp]
    \centering
    \includegraphics[width=1\linewidth]{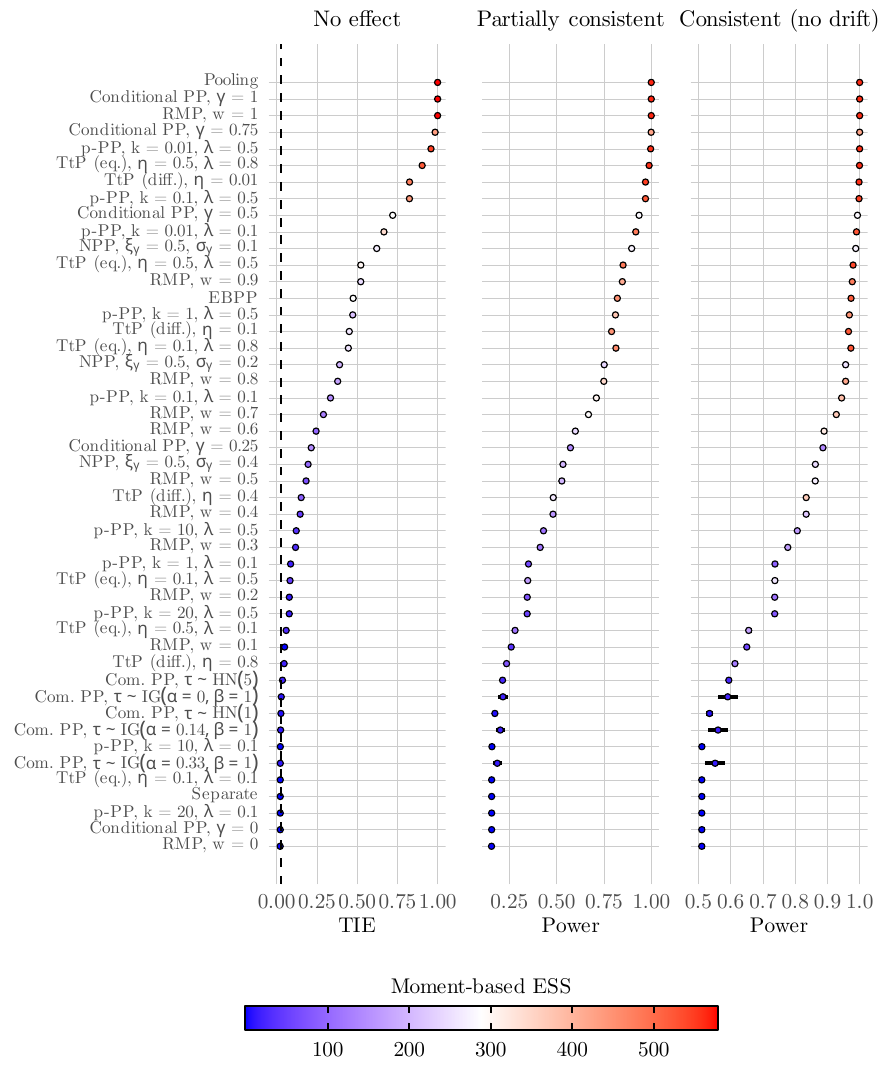}
    \caption{Probability of study success for the three main treatment effect values considered in the Belimumab case study ($N_T/2= 140$)).
    TtP (diff/eq) : test-then-pool with a test for difference/equivalence ($\eta$: significance level of the test. $\lambda$: equivalence margin ). Conditional PP : Conditional Power Prior ($\gamma$: power parameter). p-PP : p-value-based PP ($k$: shape parameter, $\lambda$: equivalence margin). EBPP: Empirical Bayes PP.
RMP : Robust Mixture Prior ($w$: weight of the informative prior component). NPP : Normalized PP ($\xi_\gamma$ and $\sigma_\gamma$ are respectively the mean and standard deviation of the Beta prior on the power parameter $\gamma$). Com. PP : Commensurate PP ($\tau$: heterogeneity parameter). Separate : separate analysis of the target trial data alone.
    }
    \label{fig:belimumab_success_proba_forest_plot_target_sample_size_per_arm_140}
 \end{figure} 

\begin{figure}[htbp]
    \centering
    \includegraphics[width=1\linewidth]{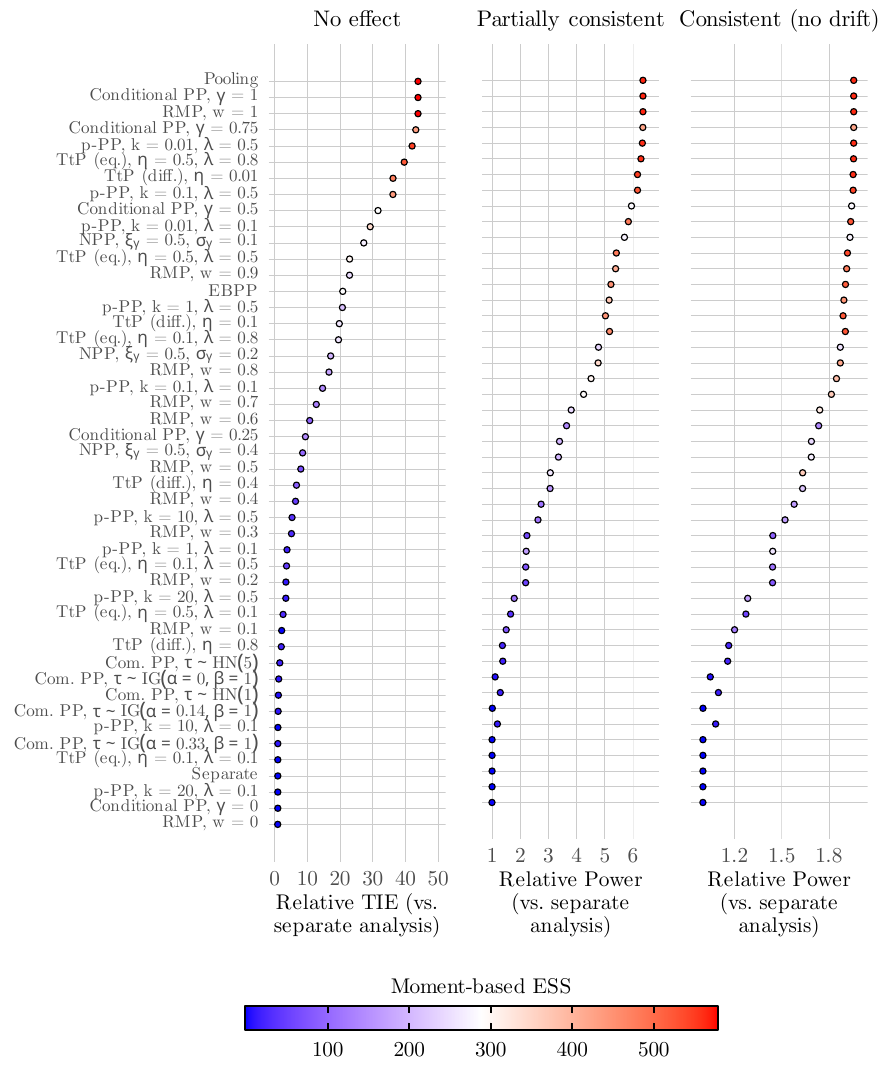}
    \caption{Probability of study success relative to the separate analysis of target study data for the three main treatment effect values considered in the Belimumab case study ($N_T/2= 140$)).
    TtP (diff/eq) : test-then-pool with a test for difference/equivalence ($\eta$: significance level of the test. $\lambda$: equivalence margin ). Conditional PP : Conditional Power Prior ($\gamma$: power parameter). p-PP : p-value-based PP ($k$: shape parameter, $\lambda$: equivalence margin). EBPP: Empirical Bayes PP.
RMP : Robust Mixture Prior ($w$: weight of the informative prior component). NPP : Normalized PP ($\xi_\gamma$ and $\sigma_\gamma$ are respectively the mean and standard deviation of the Beta prior on the power parameter $\gamma$). Com. PP : Commensurate PP ($\tau$: heterogeneity parameter). Separate : separate analysis of the target trial data alone.
    }
    \label{fig:belimumab_relative_success_proba_forest_plot_target_sample_size_per_arm_140}
 \end{figure} 
 
\begin{figure}[htbp]
    \centering
    \includegraphics[width=1\linewidth]{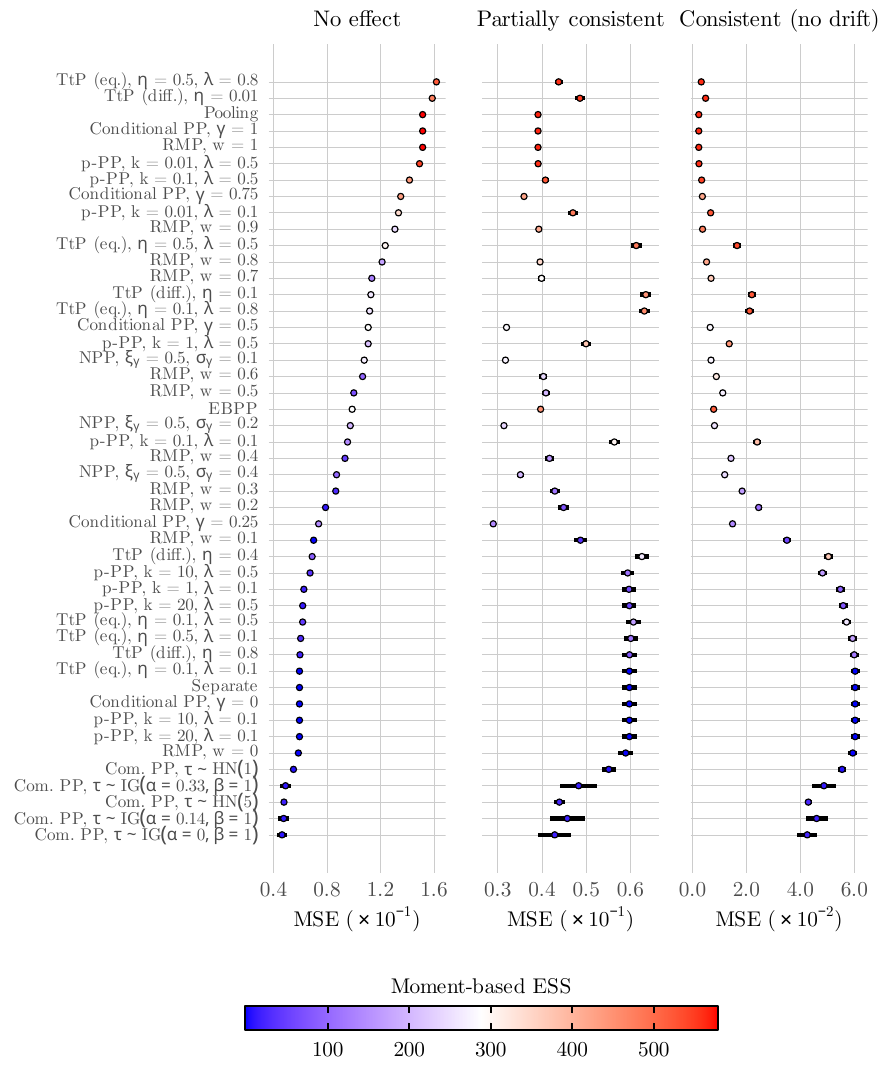}
    \caption{MSE for the three main treatment effect values considered in the Belimumab case study ($N_T/2= 140$)).
    TtP (diff/eq) : test-then-pool with a test for difference/equivalence ($\eta$: significance level of the test. $\lambda$: equivalence margin ). Conditional PP : Conditional Power Prior ($\gamma$: power parameter). p-PP : p-value-based PP ($k$: shape parameter, $\lambda$: equivalence margin). EBPP: Empirical Bayes PP.
RMP : Robust Mixture Prior ($w$: weight of the informative prior component). NPP : Normalized PP ($\xi_\gamma$ and $\sigma_\gamma$ are respectively the mean and standard deviation of the Beta prior on the power parameter $\gamma$). Com. PP : Commensurate PP ($\tau$: heterogeneity parameter). Separate : separate analysis of the target trial data alone.
    }
    \label{fig:belimumab_mse_forest_plot_target_sample_size_per_arm_140}
 \end{figure} 
 
\begin{figure}[htbp]
    \centering
    \includegraphics[width=1\linewidth]{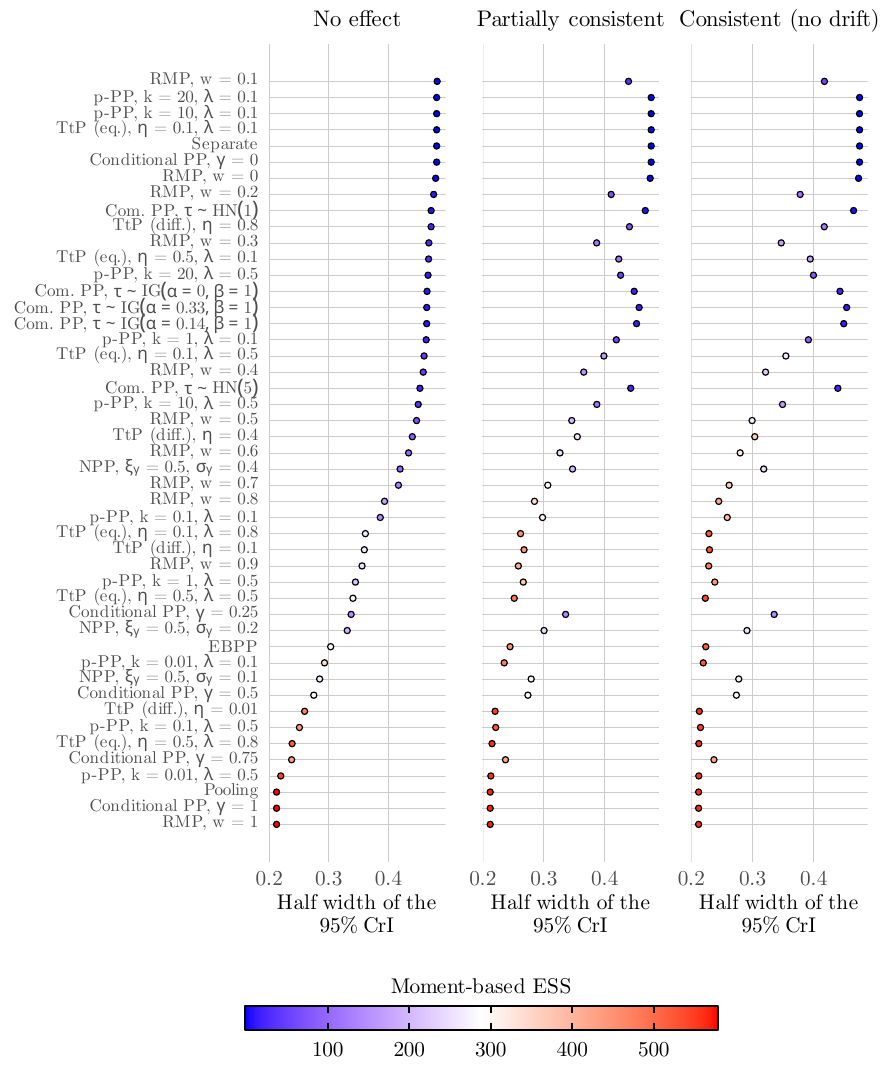}
    \caption{Precision, measured as the mean half-width of the 95\% Credible Interval,  for the three main treatment effect values considered in the Belimumab case study with a sample size per arm of 140 subjects. Error bars correspond to the 95\% CI.
    TtP (diff/eq) : test-then-pool with a test for difference/equivalence ($\eta$: significance level of the test. $\lambda$: equivalence margin ). Conditional PP : Conditional Power Prior ($\gamma$: power parameter). p-PP : p-value-based PP ($k$: shape parameter, $\lambda$: equivalence margin). EBPP: Empirical Bayes PP.
RMP : Robust Mixture Prior ($w$: weight of the informative prior component). NPP : Normalized PP ($\xi_\gamma$ and $\sigma_\gamma$ are respectively the mean and standard deviation of the Beta prior on the power parameter $\gamma$). Com. PP : Commensurate PP ($\tau$: heterogeneity parameter). Separate : separate analysis of the target trial data alone.
    }
    \label{fig:belimumab_precision_forest_plot_target_sample_size_per_arm_140}
 \end{figure}

\begin{figure}[htbp]
        \centering
        \includegraphics[width=1\linewidth]{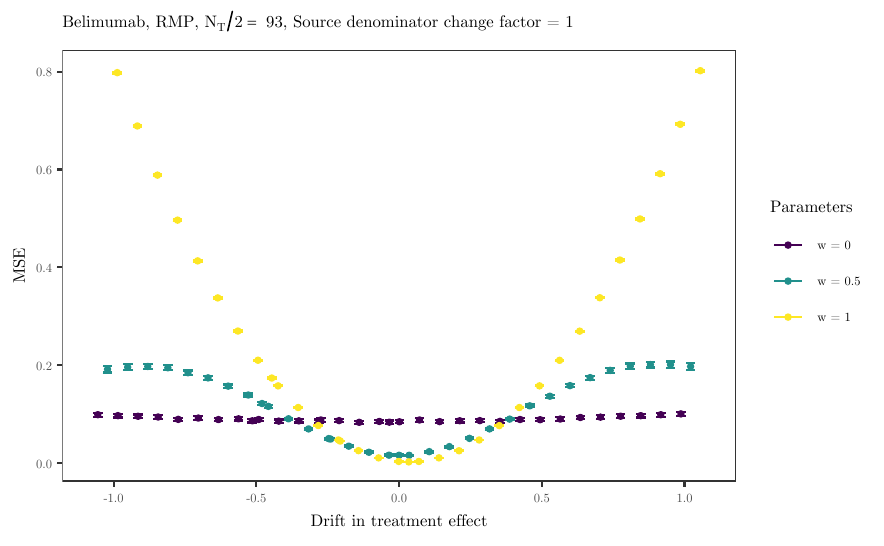}
        \caption{MSE as a function of drift for the RMP in the Belimumab case study, with a sample size per arm in the target study of 93 patients, for different values of the weight of the informative component $w$. Error bars correspond to the 95\% CI of the MSE.}
        \label{fig:belimumab_RMP_mse_vs_drift_cat_parameters_sample_size=93_source_denominator_change_factor=1}
\end{figure}

 \begin{figure}[htbp]
\centering
\includegraphics[width=1\linewidth]{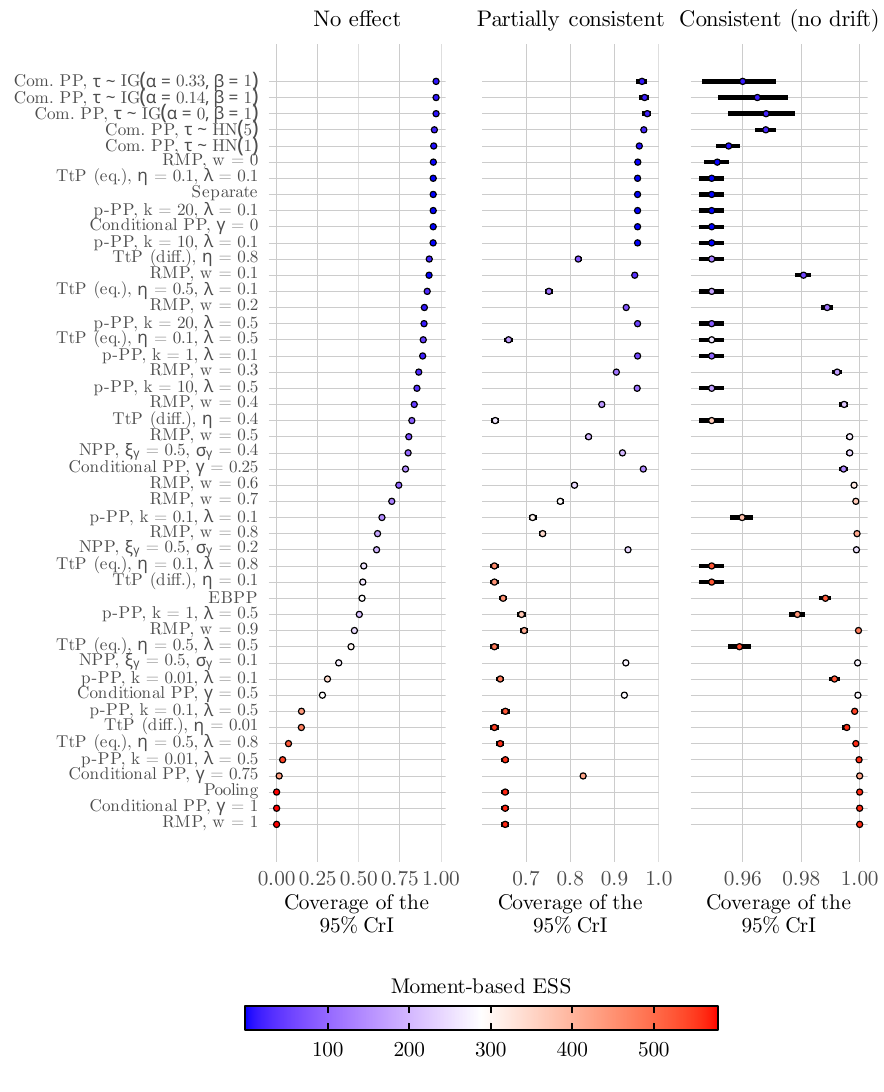}
\caption{Coverage probability of the 95\% CrI for the three main treatment effect values considered in the Belimumab case study with a sample size per arm of 140 patients. Error bars correspond to the 95\% CI on the coverage probability.
TtP (diff/eq) : test-then-pool with a test for difference/equivalence ($\eta$: significance level of the test. $\lambda$: equivalence margin ). Conditional PP : Conditional Power Prior ($\gamma$: power parameter). p-PP : p-value-based PP ($k$: shape parameter, $\lambda$: equivalence margin). EBPP: Empirical Bayes PP.
RMP : Robust Mixture Prior ($w$: weight of the informative prior component). NPP : Normalized PP ($\xi_\gamma$ and $\sigma_\gamma$ are respectively the mean and standard deviation of the Beta prior on the power parameter $\gamma$). Com. PP : Commensurate PP ($\tau$: heterogeneity parameter). Separate : separate analysis of the target trial data alone.
}
\label{fig:belimumab_coverage_forest_plot_target_sample_size_per_arm_140}
\end{figure}

\begin{table}
    \centering 
    \includegraphics[width=1\linewidth]{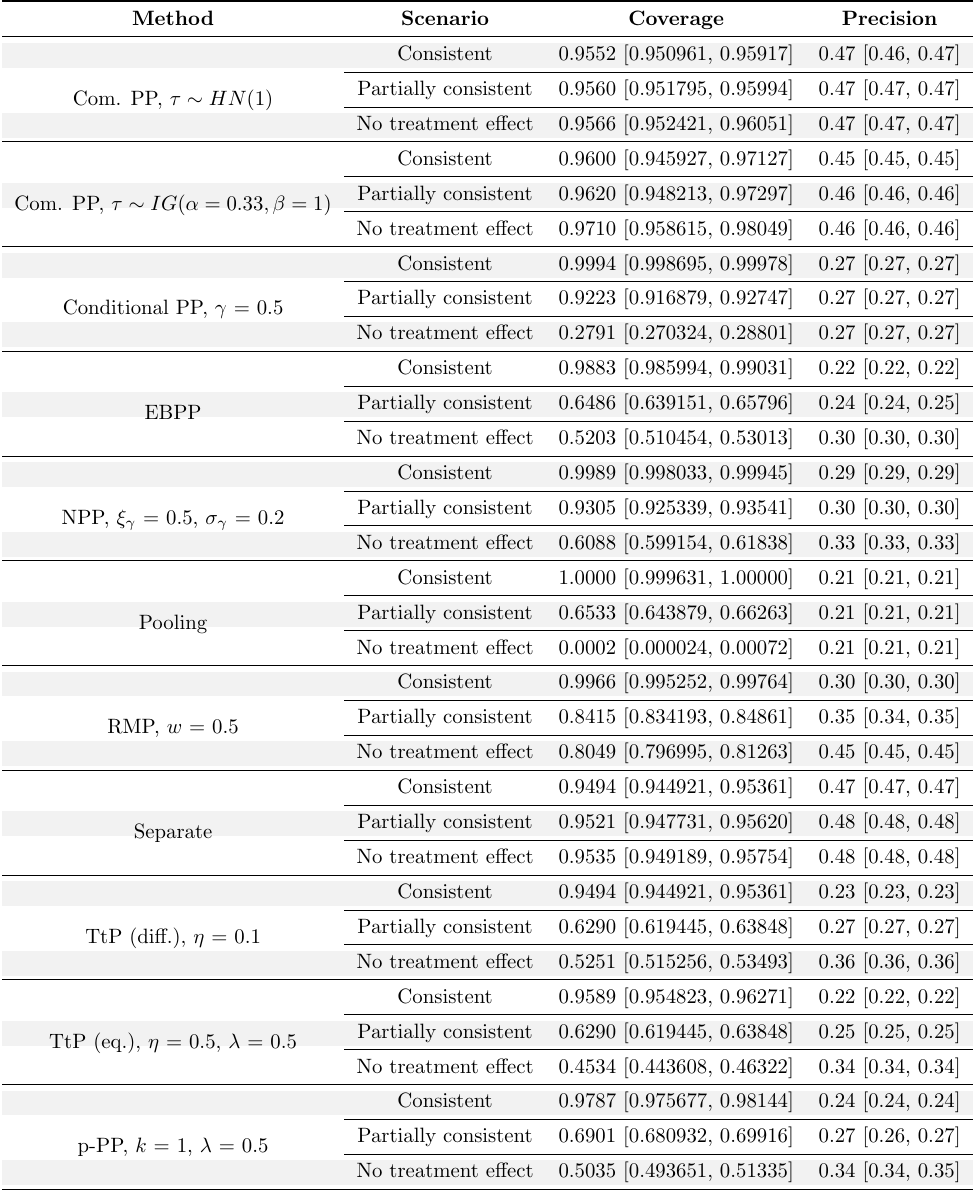}
    \caption{Precision (half-width of the CrI) and Coverage Probability, Belimumab, $N_T /2 = 140$.} \label{tab:belimumab_precision_ecp_table_target_sample_size_per_arm_140}
\end{table}

%\subfile{Tables_results/belimumab_precision_ecp_table_target_sample_size_per_arm_281_source_denominator_change_factor=1}

\clearpage
\subsection{Supplementary figures for the Mepolizumab case study (recurrent event endpoint).}

\begin{figure}[htbp]
    \centering
    \includegraphics[width=1\linewidth]{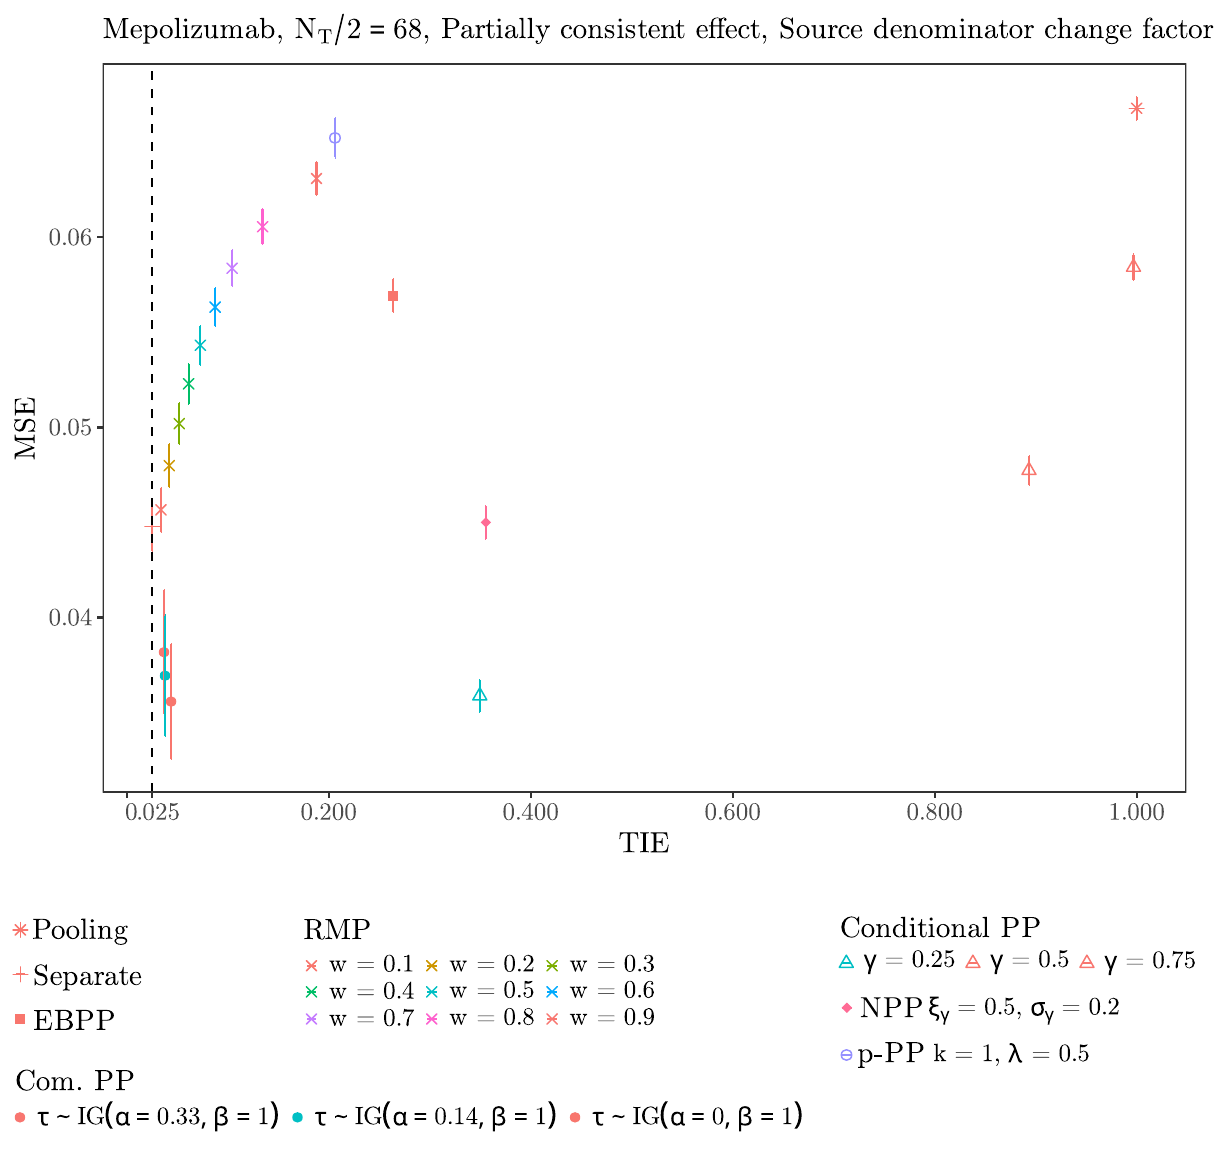}
    \caption{MSE as a function of type 1 error rate in the mepolizumab case study ($N_T/2=68$), with partially consistent treatment effect. Error bars correspond to the 95\% CI. Dashed vertical line represents the nominal type 1 error rate of $0.025$. TtP (diff/eq) : test-then-pool with a test for difference/equivalence ($\eta$: significance level of the test. $\lambda$: equivalence margin ). Conditional PP : Conditional Power Prior ($\gamma$: power parameter). p-PP : p-value-based PP ($k$: shape parameter, $\lambda$: equivalence margin). EBPP: Empirical Bayes PP.
RMP : Robust Mixture Prior ($w$: weight of the informative prior component). NPP : Normalized PP ($\xi_\gamma$ and $\sigma_\gamma$ are respectively the mean and standard deviation of the Beta prior on the power parameter $\gamma$). Com. PP : Commensurate PP ($\tau$: heterogeneity parameter). Separate : separate analysis of the target trial data alone.}
    \label{fig:teriflunomide_mse_vs_tie_sample_size=68_treatment_effect=partially_consistent}
\end{figure}

\begin{figure}[htbp]
    \centering
    \includegraphics[width=1\linewidth]{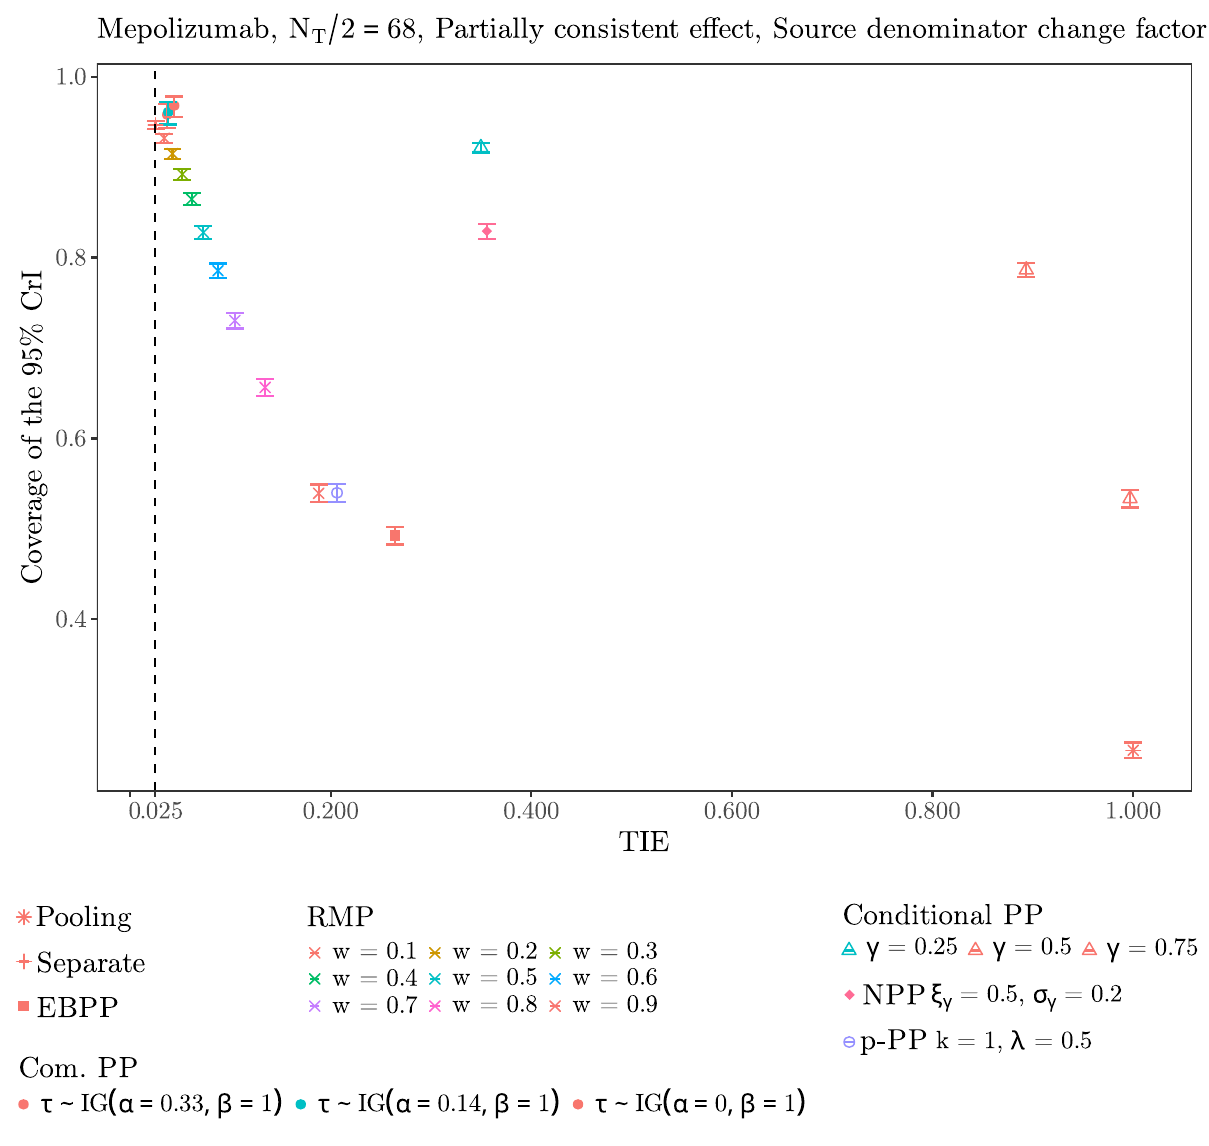}
    \caption{Coverage of the 95\% Confidence Interval as a function of type 1 error rate in the Mepolizumab case study with a sample size per arm of $68$, across all the methods and parameters, without treatment effect. Error bars correspond to the 95\% CI of the Coverage and type 1 error rate. Dashed vertical line represents the nominal type 1 error rate of $0.025$.
    TtP (diff/eq) : test-then-pool with a test for difference/equivalence ($\eta$: significance level of the test. $\lambda$: equivalence margin ). Conditional PP : Conditional Power Prior ($\gamma$: power parameter). p-PP : p-value-based PP ($k$: shape parameter, $\lambda$: equivalence margin). EBPP: Empirical Bayes PP.
RMP : Robust Mixture Prior ($w$: weight of the informative prior component). NPP : Normalized PP ($\xi_\gamma$ and $\sigma_\gamma$ are respectively the mean and standard deviation of the Beta prior on the power parameter $\gamma$). Com. PP : Commensurate PP ($\tau$: heterogeneity parameter). Separate : separate analysis of the target trial data alone.
}    \label{fig:mepolizumab_coverage_vs_tie_sample_size=68_treatment_effect=partially_consistent_source_denominator_change_factor=}
\end{figure}

\begin{figure}
    \centering
    \includegraphics[width=1\linewidth]{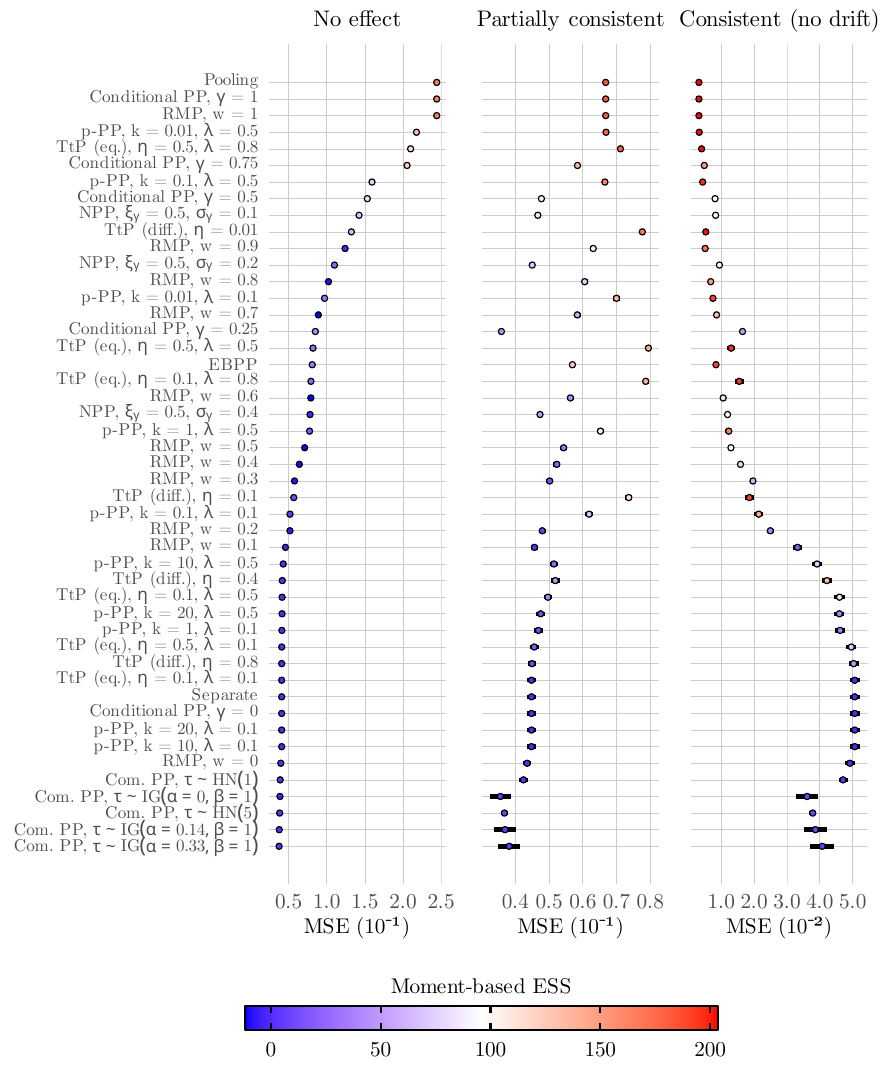}
    \caption{MSE for the three main treatment effect values considered in the Mepolizumab case study ($N_T/2=68$).
    TtP (diff/eq) : test-then-pool with a test for difference/equivalence ($\eta$: significance level of the test. $\lambda$: equivalence margin ). Conditional PP : Conditional Power Prior ($\gamma$: power parameter). p-PP : p-value-based PP ($k$: shape parameter, $\lambda$: equivalence margin). EBPP: Empirical Bayes PP.
RMP : Robust Mixture Prior ($w$: weight of the informative prior component). NPP : Normalized PP ($\xi_\gamma$ and $\sigma_\gamma$ are respectively the mean and standard deviation of the Beta prior on the power parameter $\gamma$). Com. PP : Commensurate PP ($\tau$: heterogeneity parameter). Separate : separate analysis of the target trial data alone.}
    \label{fig:mepolizumab_mse_forest_plot_target_sample_size_per_arm_68}
\end{figure}

\begin{figure}
    \centering
    \includegraphics[width=1\linewidth]{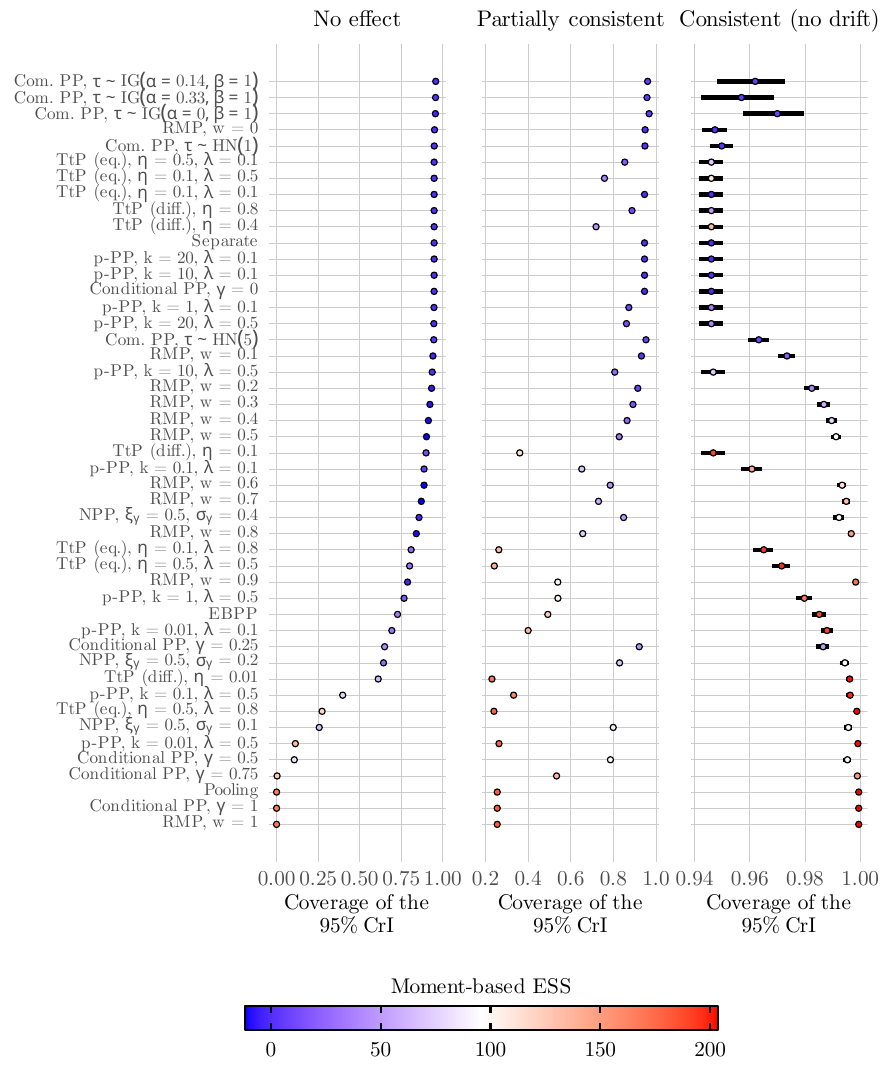}
    \caption{Empirical coverage probability  for the three main treatment effect values considered in the Mepolizumab case study ($N_T/2=68$)). Error bars correspond to the 95\% CI.
    TtP (diff/eq) : test-then-pool with a test for difference/equivalence ($\eta$: significance level of the test. $\lambda$: equivalence margin ). Conditional PP : Conditional Power Prior ($\gamma$: power parameter). p-PP : p-value-based PP ($k$: shape parameter, $\lambda$: equivalence margin). EBPP: Empirical Bayes PP.
RMP : Robust Mixture Prior ($w$: weight of the informative prior component). NPP : Normalized PP ($\xi_\gamma$ and $\sigma_\gamma$ are respectively the mean and standard deviation of the Beta prior on the power parameter $\gamma$). Com. PP : Commensurate PP ($\tau$: heterogeneity parameter). Separate : separate analysis of the target trial data alone.
}
    \label{fig:mepolizumab_coverage_forest_plot_target_sample_size_per_arm_68}
\end{figure}

\begin{figure}
    \centering
    \includegraphics[width=1\linewidth]{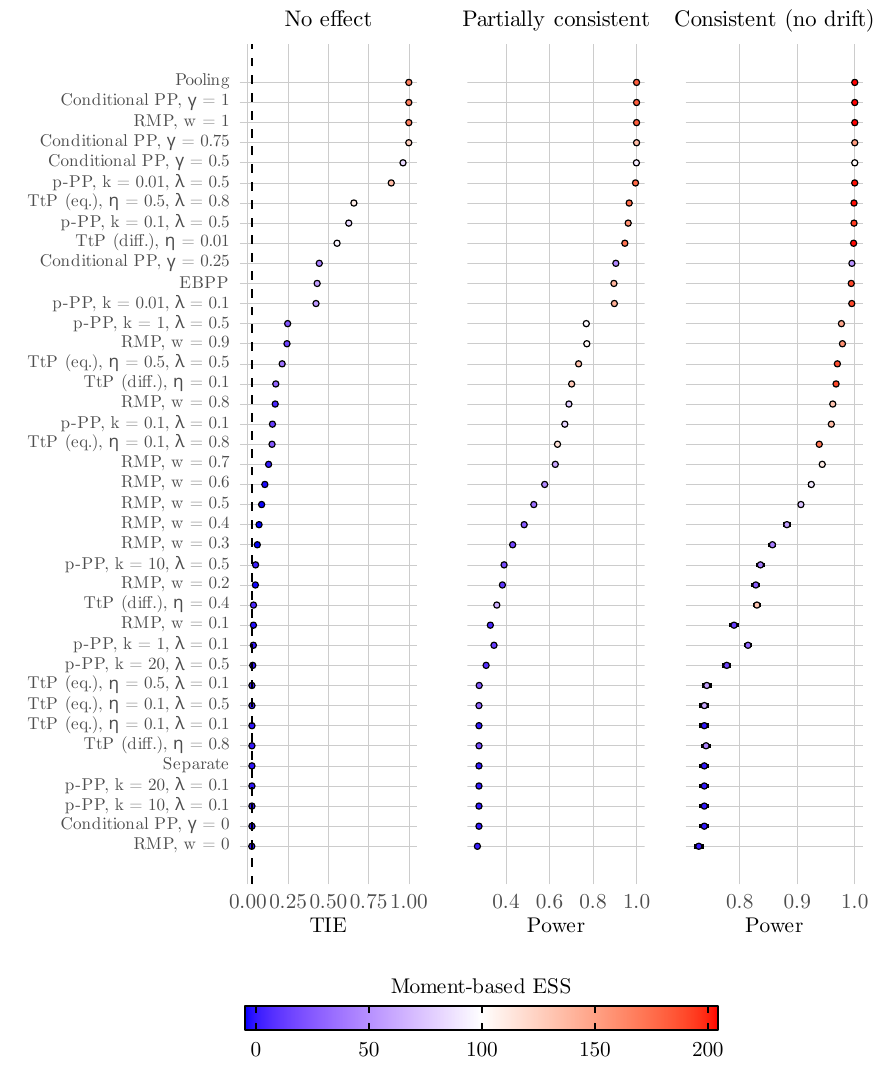}
    \caption{Probability of study success for the three main treatment effect values considered in the Mepolizumab case study ($N_T/2=45$). TtP (diff/eq) : test-then-pool with a test for difference/equivalence ($\eta$: significance level of the test. $\lambda$: equivalence margin ). Conditional PP : Conditional Power Prior ($\gamma$: power parameter). p-PP : p-value-based PP ($k$: shape parameter, $\lambda$: equivalence margin). EBPP: Empirical Bayes PP.
RMP : Robust Mixture Prior ($w$: weight of the informative prior component). NPP : Normalized PP ($\xi_\gamma$ and $\sigma_\gamma$ are respectively the mean and standard deviation of the Beta prior on the power parameter $\gamma$). Com. PP : Commensurate PP ($\tau$: heterogeneity parameter). Separate : separate analysis of the target trial data alone.}    \label{fig:mepolizumab_success_proba_forest_plot_target_sample_size_per_arm_45}
\end{figure}

 \begin{figure}
     \centering
     \includegraphics[width=1\linewidth]{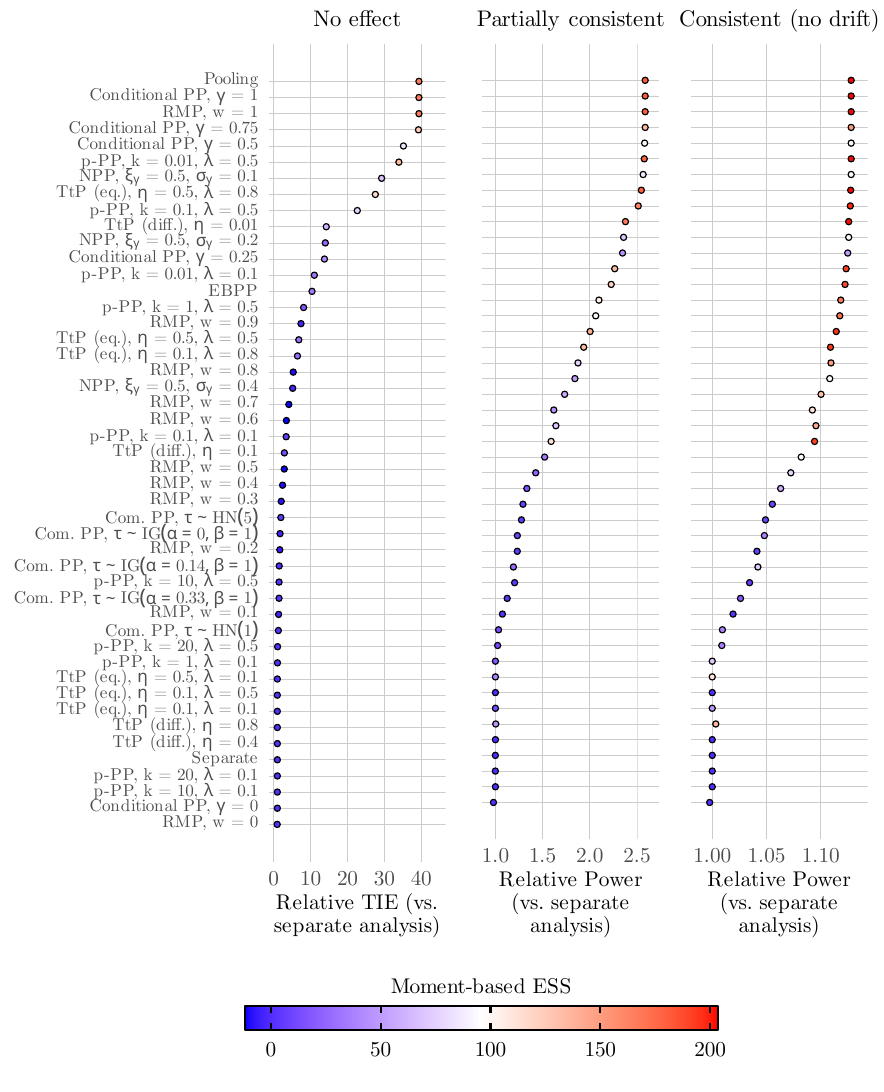}
     \caption{Probability of study success for the different methods for the three main treatment effect values considered in the Mepolizumab case study ($N_T/2=68$), relative to the probability of success in the case of a separate analysis. TtP (diff/eq) : test-then-pool with a test for difference/equivalence ($\eta$: significance level of the test. $\lambda$: equivalence margin ). Conditional PP : Conditional Power Prior ($\gamma$: power parameter). p-PP : p-value-based PP ($k$: shape parameter, $\lambda$: equivalence margin). EBPP: Empirical Bayes PP.
RMP : Robust Mixture Prior ($w$: weight of the informative prior component). NPP : Normalized PP ($\xi_\gamma$ and $\sigma_\gamma$ are respectively the mean and standard deviation of the Beta prior on the power parameter $\gamma$). Com. PP : Commensurate PP ($\tau$: heterogeneity parameter). Separate : separate analysis of the target trial data alone.}     \label{fig:mepolizumab_relative_success_proba_forest_plot_target_sample_size_per_arm_68}
 \end{figure}

\clearpage
\subsection{Supplementary figures for the Teriflunomide case study (time-to-event endpoint).}

\begin{figure}[htbp]
    \centering
    \includegraphics[width=1\linewidth]{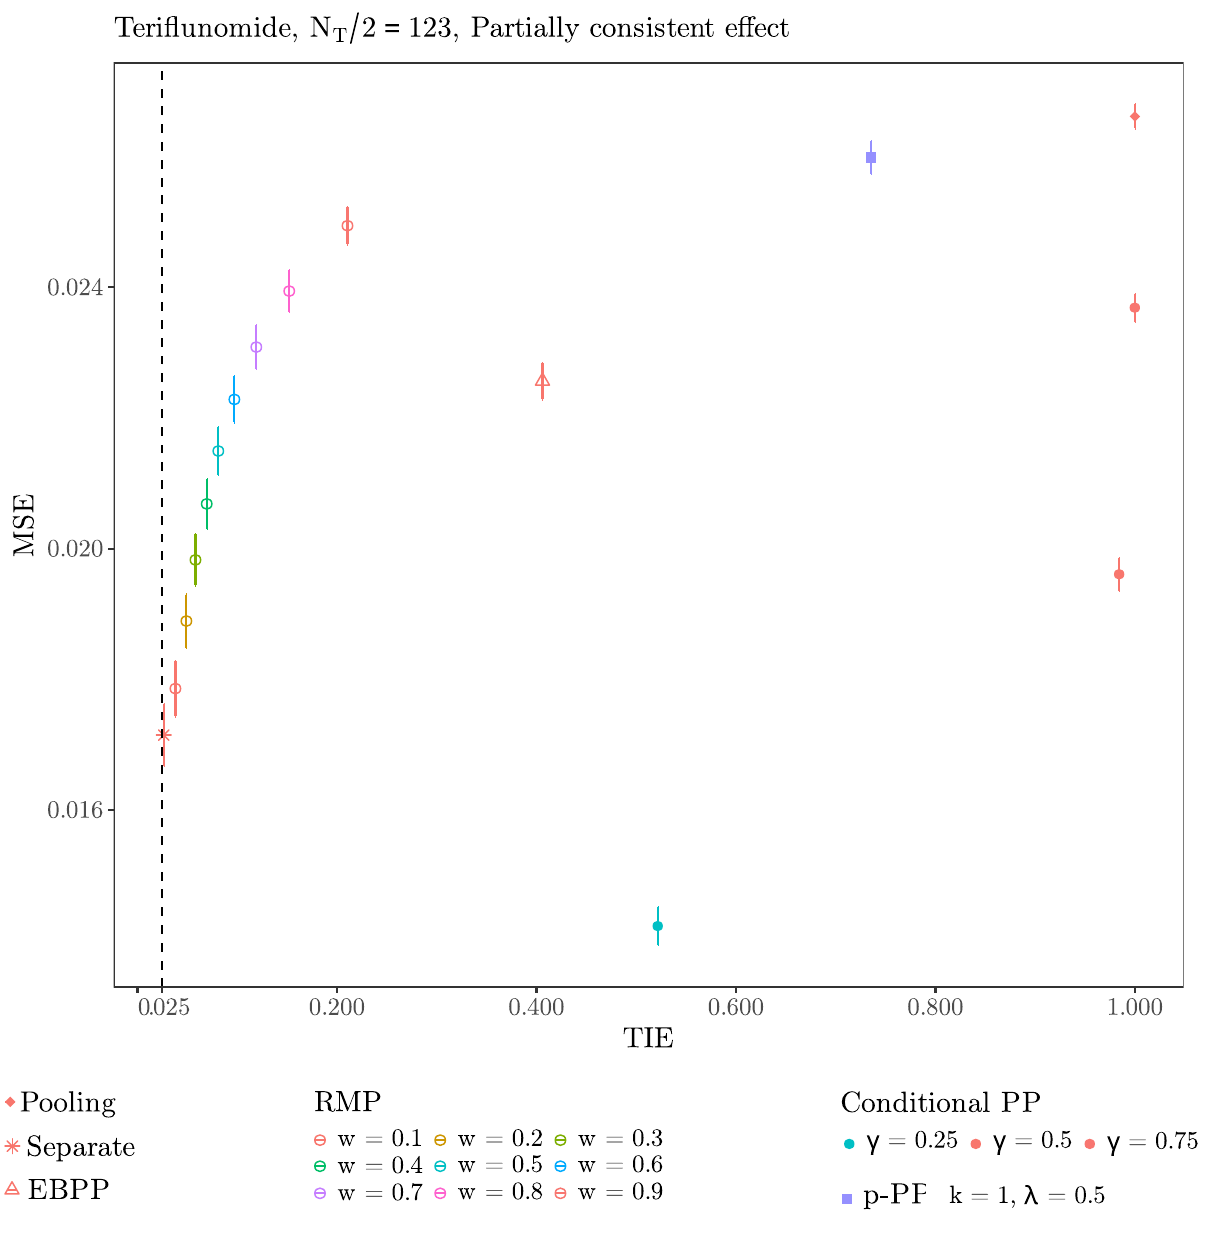}
    \caption{MSE as a function of type 1 error rate in the teriflunomide case study ($N_T/2=123$), with partially consistent treatment effect. Error bars correspond to the 95\% CI. Dashed vertical line represents the nominal type 1 error rate of $0.025$. TtP (diff/eq) : test-then-pool with a test for difference/equivalence ($\eta$: significance level of the test. $\lambda$: equivalence margin ). Conditional PP : Conditional Power Prior ($\gamma$: power parameter). p-PP : p-value-based PP ($k$: shape parameter, $\lambda$: equivalence margin). EBPP: Empirical Bayes PP.
RMP : Robust Mixture Prior ($w$: weight of the informative prior component). NPP : Normalized PP ($\xi_\gamma$ and $\sigma_\gamma$ are respectively the mean and standard deviation of the Beta prior on the power parameter $\gamma$). Com. PP : Commensurate PP ($\tau$: heterogeneity parameter). Separate : separate analysis of the target trial data alone.}
    \label{fig:teriflunomide_mse_vs_tie_sample_size=123treatment_effect=partially_consistent}
\end{figure}

\begin{figure}[htbp]
    \centering
    \includegraphics[width=1\linewidth]{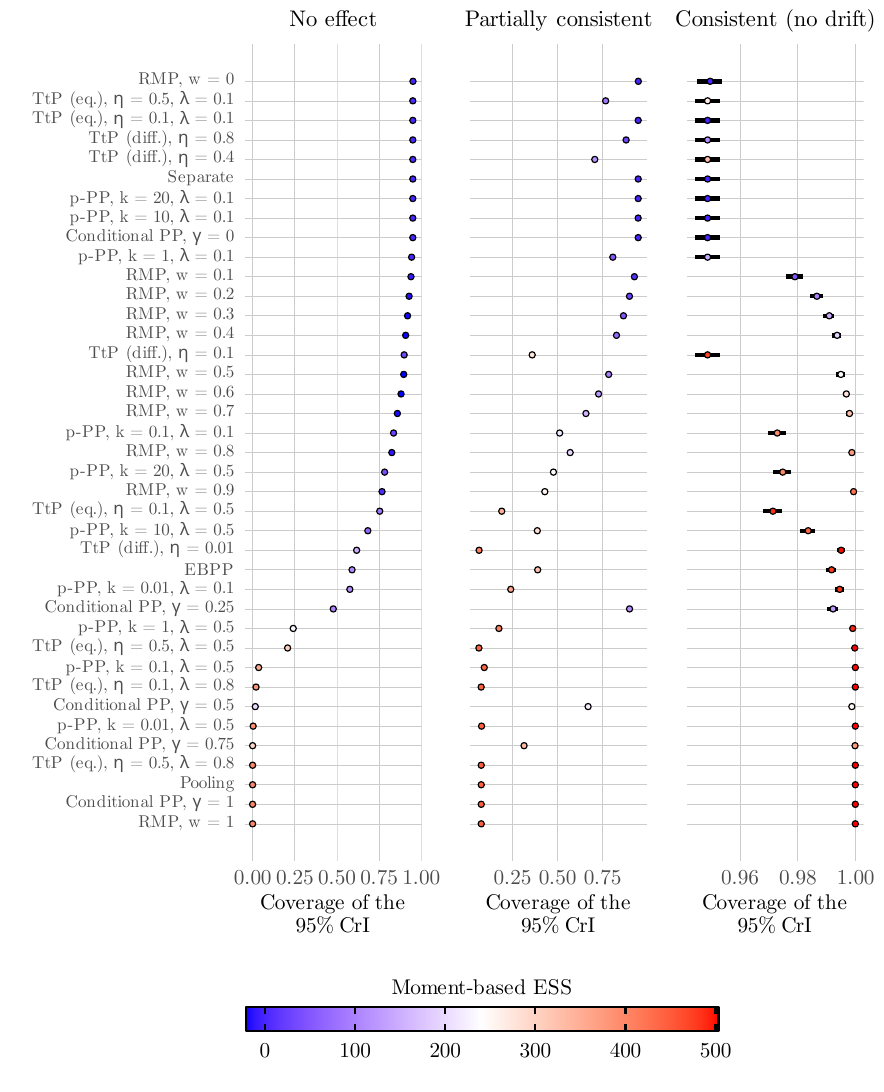}
    \caption{Coverage of the 95\% Confidence Interval as a function of type 1 error rate in the Teriflunomide case study with a sample size per arm of $123$, across all the methods and parameters, without treatment effect. The target to source standard deviation ratio is $1$. Error bars correspond to the 95\% CI. Dashed vertical line represents the nominal type 1 error rate of $0.025$. TtP (diff) : test-then-pool with a test for difference.  $\eta$ is the significance level of the test. TtP (eq) : test-then-pool with a test for equivalence. $\lambda$ is an equivalence margin for the test. p-PP : p-value-based Power Prior.  $k$ is a shape parameter. $\lambda$ is an equivalence margin for the test. EBPP: Empirical Bayes Power Prior. RMP : Robust Mixture Prior. $w$ is the prior weight of the informative prior component. Conditional PP : Conditional Power Prior. $\gamma$ is the power parameter. NPP : Normalized Power Prior. $\xi_\gamma$ and $\sigma_\gamma$ are respectively the mean and standard deviation of the Beta prior on the power parameter $\gamma$. Com. PP : Commensurate Power Prior. $\tau$ is an heterogeneity parameter.  Separate : separate analysis of the target trial data.}
    \label{fig:teriflunomide_coverage_forest_plot_target_sample_size_per_arm_123}
\end{figure} 

\begin{figure}
    \centering
    \includegraphics[width=1\linewidth]{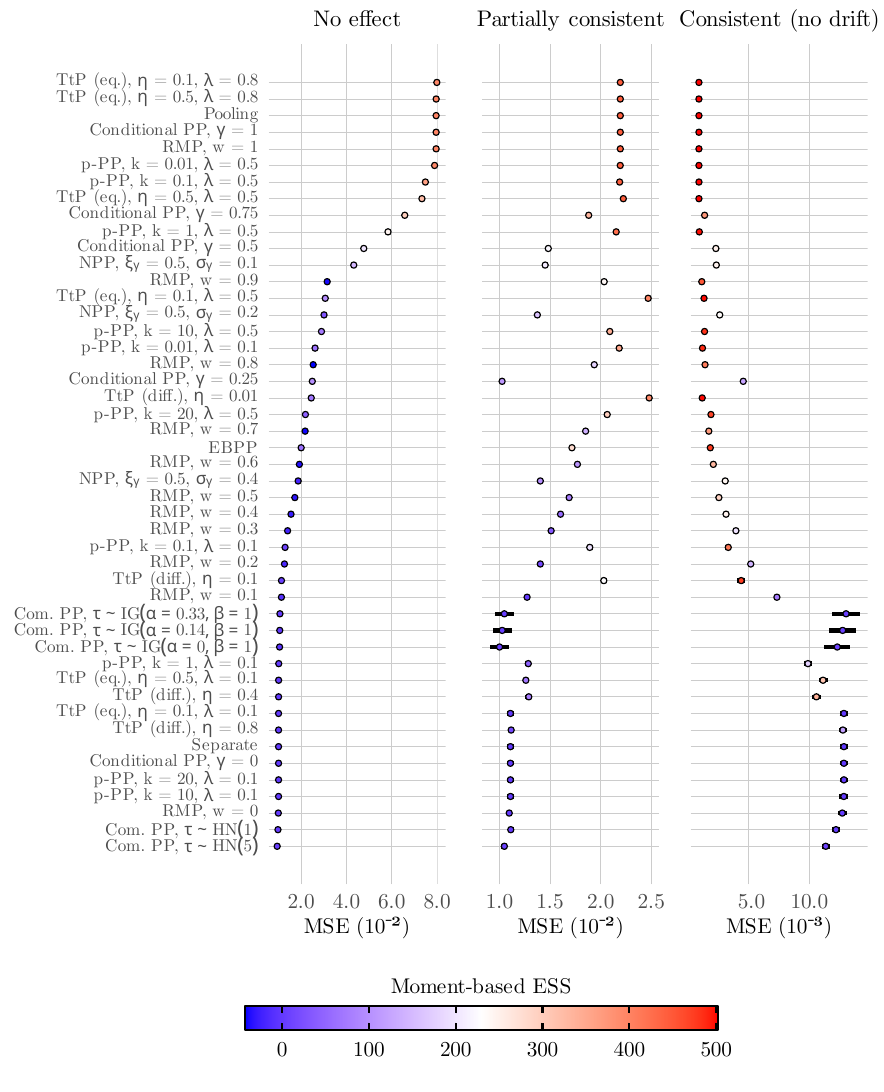}
    \caption{MSE for the three main treatment effect values considered in the Teriflunomide case study ($N_T/2 = 185$). TtP (diff/eq) : test-then-pool with a test for difference/equivalence ($\eta$: significance level of the test. $\lambda$: equivalence margin ). Conditional PP : Conditional Power Prior ($\gamma$: power parameter). p-PP : p-value-based PP ($k$: shape parameter, $\lambda$: equivalence margin). EBPP: Empirical Bayes PP.
RMP : Robust Mixture Prior ($w$: weight of the informative prior component). NPP : Normalized PP ($\xi_\gamma$ and $\sigma_\gamma$ are respectively the mean and standard deviation of the Beta prior on the power parameter $\gamma$). Com. PP : Commensurate PP ($\tau$: heterogeneity parameter). Separate : separate analysis of the target trial data alone.}    \label{fig:teriflunomide_mse_forest_plot_target_sample_size_per_arm_185}
\end{figure}
\clearpage

 \begin{figure}
     \centering
     \includegraphics[width=1\linewidth]{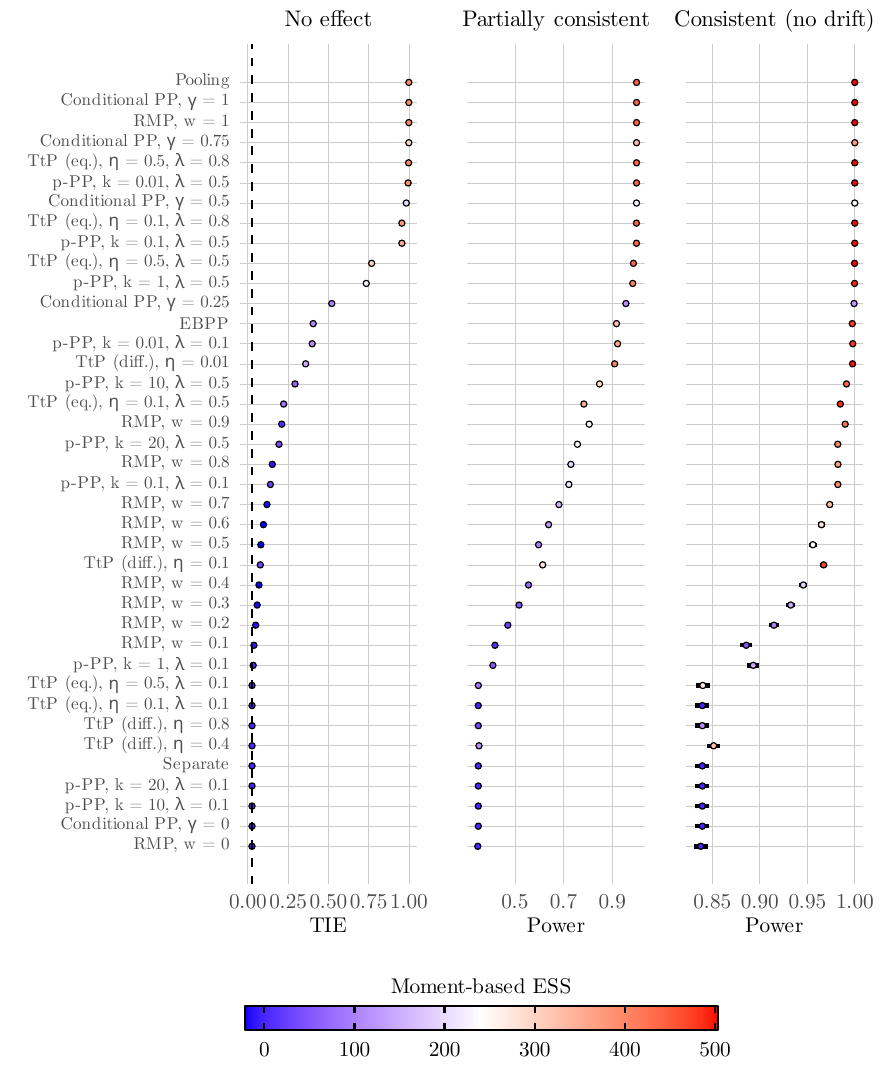}
     \caption{Probability of study success  for the three main treatment effect values considered in the Teriflunomide case study ($N_T/2 = 123$). TtP (diff/eq) : test-then-pool with a test for difference/equivalence ($\eta$: significance level of the test. $\lambda$: equivalence margin ). Conditional PP : Conditional Power Prior ($\gamma$: power parameter). p-PP : p-value-based PP ($k$: shape parameter, $\lambda$: equivalence margin). EBPP: Empirical Bayes PP.
RMP : Robust Mixture Prior ($w$: weight of the informative prior component). NPP : Normalized PP ($\xi_\gamma$ and $\sigma_\gamma$ are respectively the mean and standard deviation of the Beta prior on the power parameter $\gamma$). Com. PP : Commensurate PP ($\tau$: heterogeneity parameter). Separate : separate analysis of the target trial data alone.}     \label{fig:teriflunomide_success_proba_forest_plot_target_sample_size_per_arm_123}
 \end{figure}

 \begin{figure}
     \centering
     \includegraphics[width=1\linewidth]{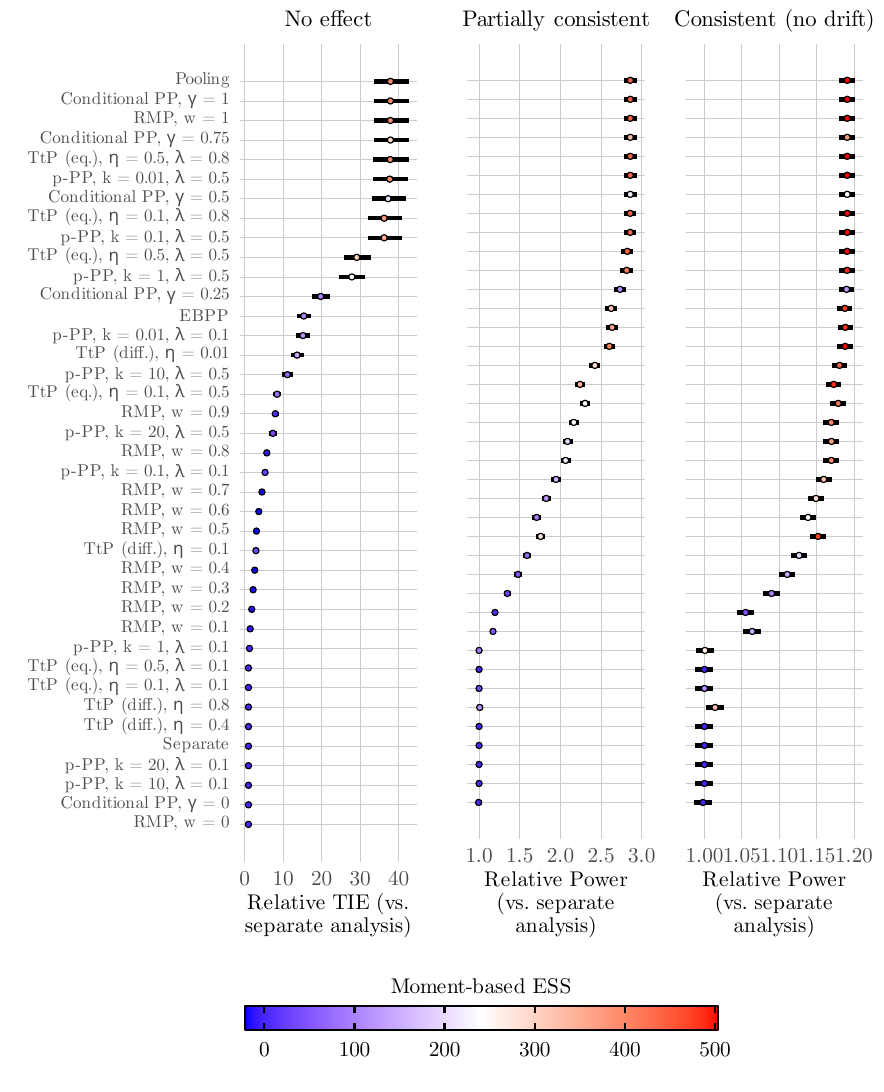}
     \caption{Probability of study success  for the three main treatment effect values considered in the Teriflunomide case study ($N_T/2 = 123$), relative to the probability of success of a separate analysis. TtP (diff/eq) : test-then-pool with a test for difference/equivalence ($\eta$: significance level of the test. $\lambda$: equivalence margin ). Conditional PP : Conditional Power Prior ($\gamma$: power parameter). p-PP : p-value-based PP ($k$: shape parameter, $\lambda$: equivalence margin). EBPP: Empirical Bayes PP.
RMP : Robust Mixture Prior ($w$: weight of the informative prior component). NPP : Normalized PP ($\xi_\gamma$ and $\sigma_\gamma$ are respectively the mean and standard deviation of the Beta prior on the power parameter $\gamma$). Com. PP : Commensurate PP ($\tau$: heterogeneity parameter). Separate : separate analysis of the target trial data alone.}     \label{fig:teriflunomide_relative_success_proba_forest_plot_target_sample_size_per_arm_123}
 \end{figure}

\clearpage
\subsection{Supplementary figures for the Aprepitant case study (binary endpoint).}

\begin{figure}[htbp]
    \centering
    \includegraphics[width=1\linewidth]{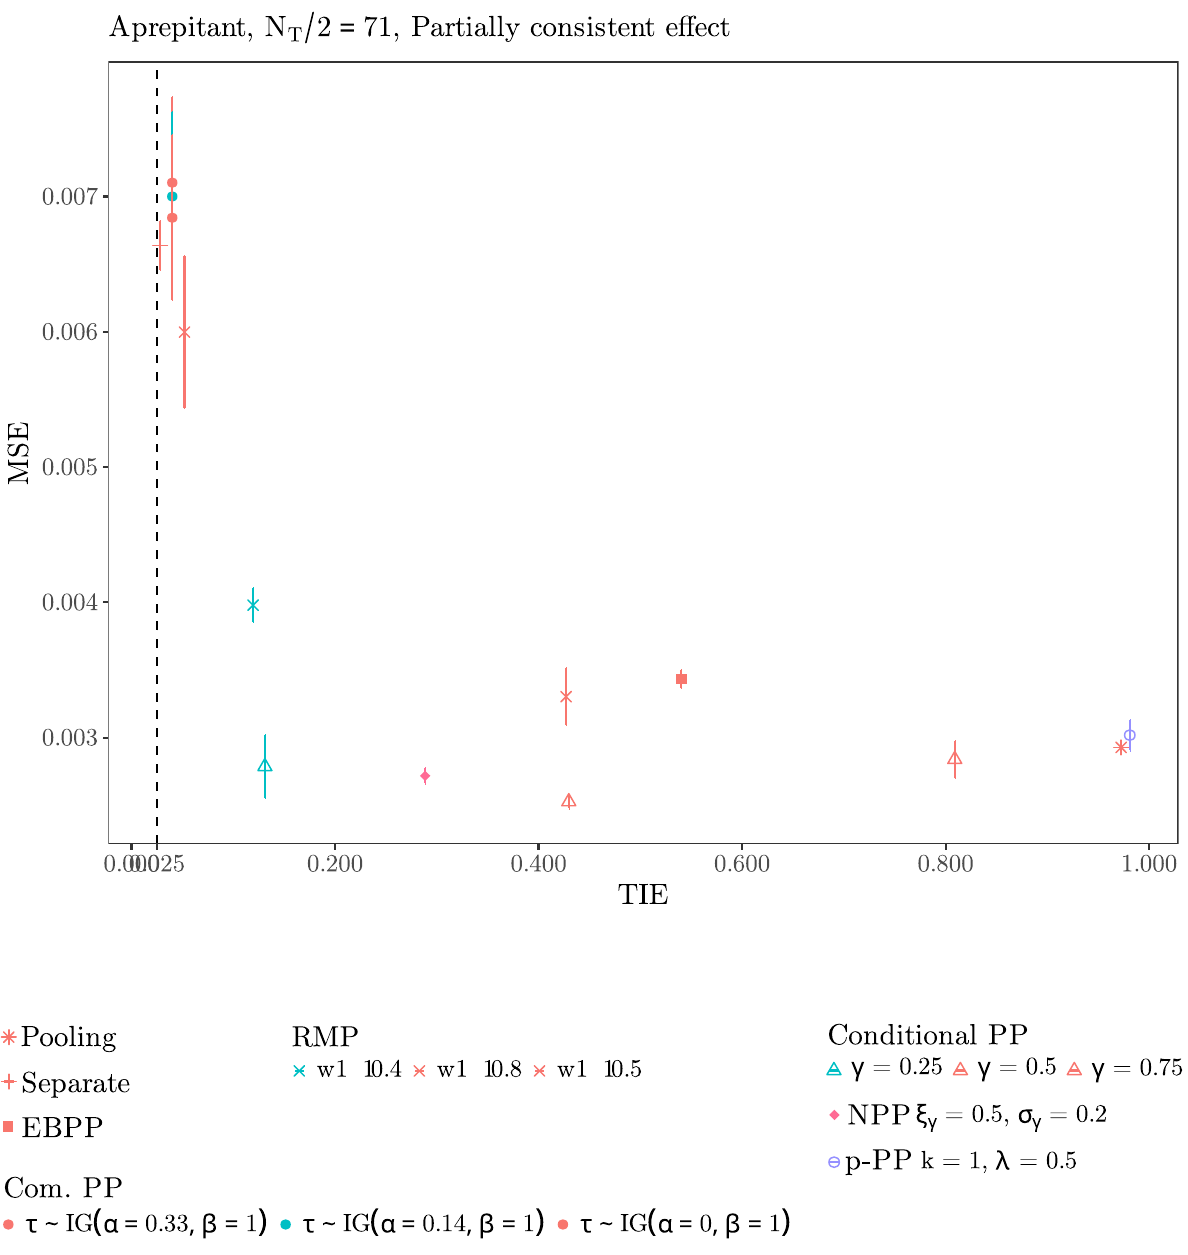}
    \caption{MSE as a function of type 1 error rate in the aprepitant case study ($N_T/2=71$), with partially consistent treatment effect. Error bars correspond to the 95\% CI. Dashed vertical line represents the nominal type 1 error rate of $0.025$. TtP (diff/eq) : test-then-pool with a test for difference/equivalence ($\eta$: significance level of the test. $\lambda$: equivalence margin ). Conditional PP : Conditional Power Prior ($\gamma$: power parameter). p-PP : p-value-based PP ($k$: shape parameter, $\lambda$: equivalence margin). EBPP: Empirical Bayes PP.
RMP : Robust Mixture Prior ($w$: weight of the informative prior component). NPP : Normalized PP ($\xi_\gamma$ and $\sigma_\gamma$ are respectively the mean and standard deviation of the Beta prior on the power parameter $\gamma$). Com. PP : Commensurate PP ($\tau$: heterogeneity parameter). Separate : separate analysis of the target trial data alone.}
    \label{fig:aprepitant_mse_vs_tie_sample_size=71_treatment_effect=partially_consistent}
\end{figure}

\begin{figure}[htpb]
    \centering
    \includegraphics[width=1\linewidth]{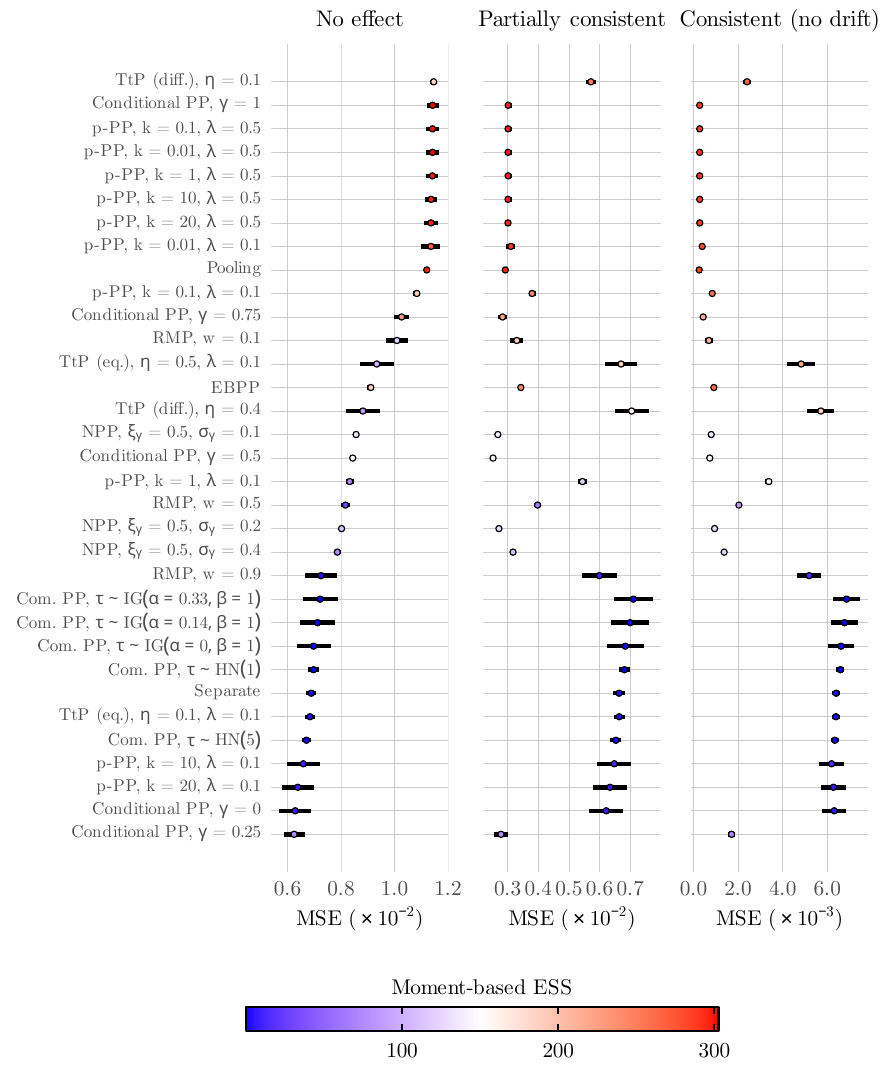}
    \caption{MSE  for the three main treatment effect values considered in the Aprepitant case study with a sample size per arm of 143 subjects. TtP (diff/eq) : test-then-pool with a test for difference/equivalence ($\eta$: significance level of the test. $\lambda$: equivalence margin ). Conditional PP : Conditional Power Prior ($\gamma$: power parameter). p-PP : p-value-based PP ($k$: shape parameter, $\lambda$: equivalence margin). EBPP: Empirical Bayes PP.
RMP : Robust Mixture Prior ($w$: weight of the informative prior component). NPP : Normalized PP ($\xi_\gamma$ and $\sigma_\gamma$ are respectively the mean and standard deviation of the Beta prior on the power parameter $\gamma$). Com. PP : Commensurate PP ($\tau$: heterogeneity parameter). Separate : separate analysis of the target trial data alone.} \label{fig:aprepitant_mse_forest_plot_target_sample_size_per_arm_71}
\end{figure}

 \begin{figure}[htpb]
    \centering
    \includegraphics[width=1\linewidth]{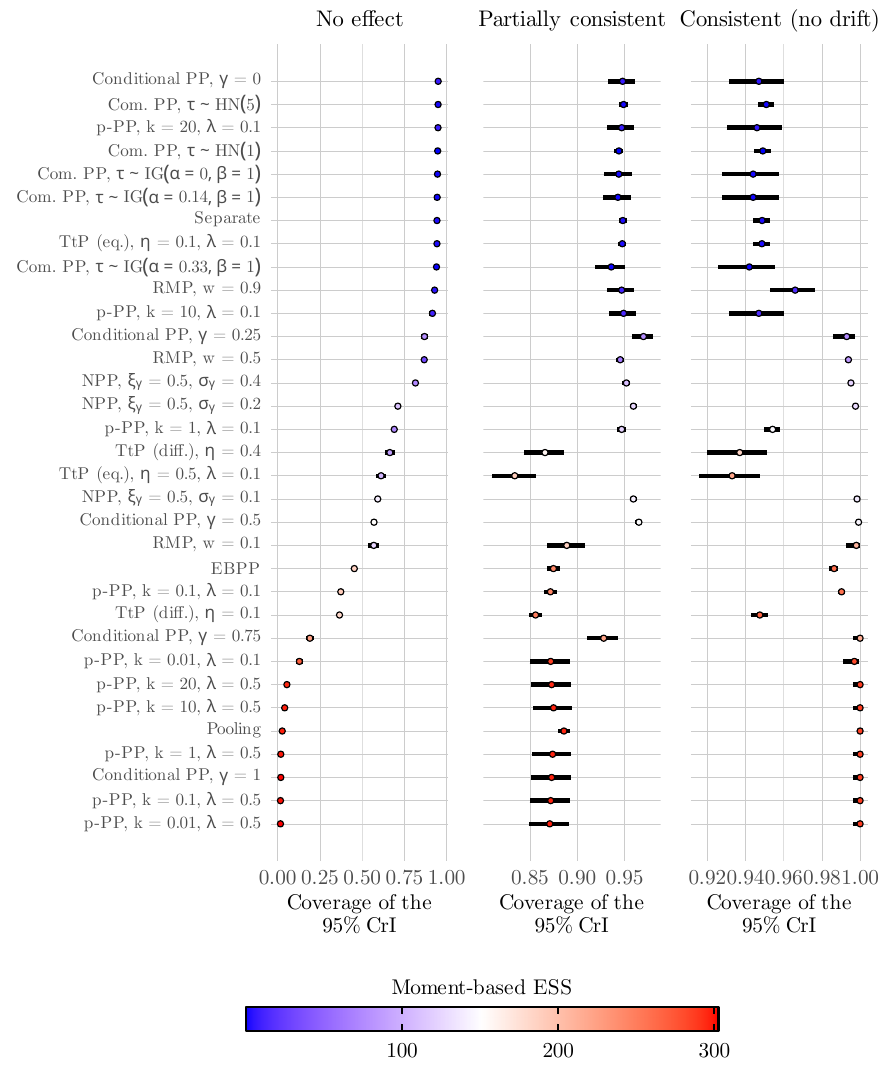}
    \caption{Empirical coverage of the 95\% CrI for the three main treatment effect values considered in the Aprepitant case study with a sample size per arm of 143 subjects. TtP (diff/eq) : test-then-pool with a test for difference/equivalence ($\eta$: significance level of the test. $\lambda$: equivalence margin ). Conditional PP : Conditional Power Prior ($\gamma$: power parameter). p-PP : p-value-based PP ($k$: shape parameter, $\lambda$: equivalence margin). EBPP: Empirical Bayes PP.
RMP : Robust Mixture Prior ($w$: weight of the informative prior component). NPP : Normalized PP ($\xi_\gamma$ and $\sigma_\gamma$ are respectively the mean and standard deviation of the Beta prior on the power parameter $\gamma$). Com. PP : Commensurate PP ($\tau$: heterogeneity parameter). Separate : separate analysis of the target trial data alone.} \label{fig:aprepitant_coverage_forest_plot_target_sample_size_per_arm_71}
\end{figure}

  \begin{figure}[htpb]
     \centering
     \includegraphics[width=1\linewidth]{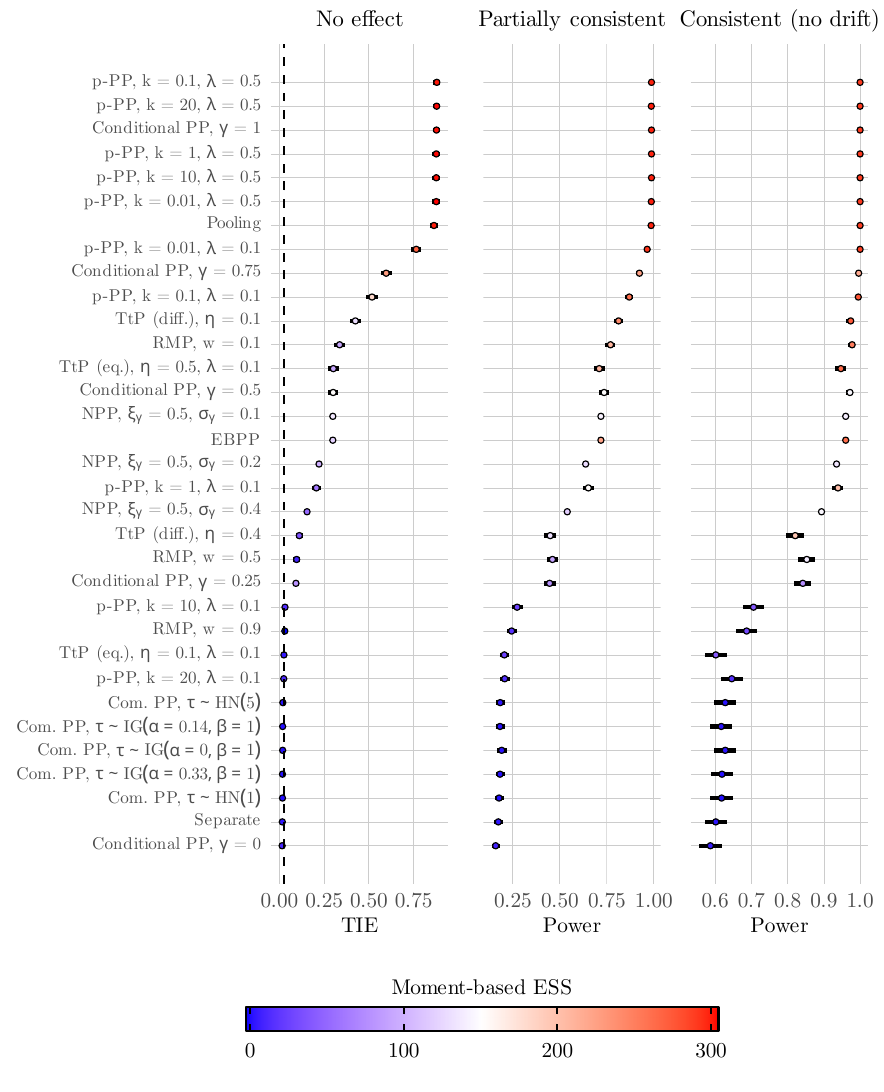}
     \caption{Probability of study success for the three main treatment effect values considered in the Aprepitant case study ($N_T/2 = 143$). TtP (diff/eq) : test-then-pool with a test for difference/equivalence ($\eta$: significance level of the test. $\lambda$: equivalence margin ). Conditional PP : Conditional Power Prior ($\gamma$: power parameter). p-PP : p-value-based PP ($k$: shape parameter, $\lambda$: equivalence margin). EBPP: Empirical Bayes PP.
RMP : Robust Mixture Prior ($w$: weight of the informative prior component). NPP : Normalized PP ($\xi_\gamma$ and $\sigma_\gamma$ are respectively the mean and standard deviation of the Beta prior on the power parameter $\gamma$). Com. PP : Commensurate PP ($\tau$: heterogeneity parameter). Separate : separate analysis of the target trial data alone.} \label{fig:aprepitant_success_proba_forest_plot_target_sample_size_per_arm_143}
 \end{figure}

 \begin{figure}[htpb]
     \centering
     \includegraphics[width=1\linewidth]{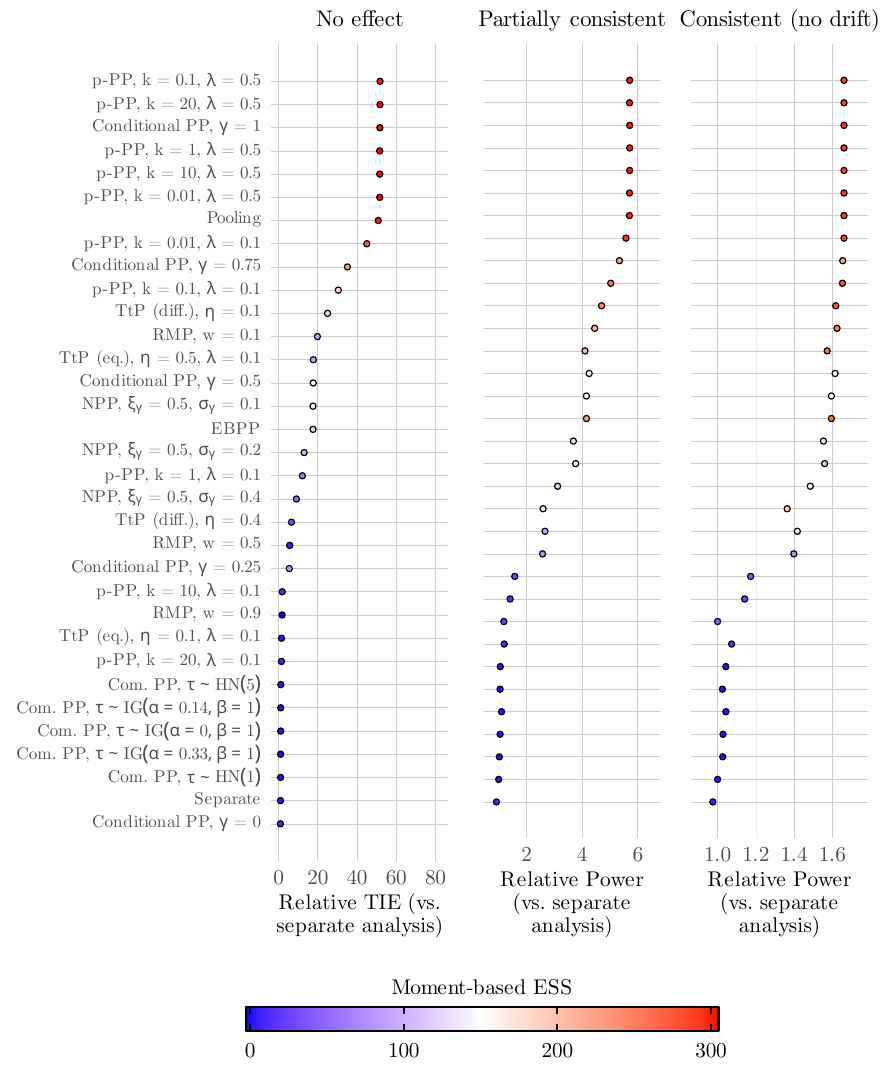}
     \caption{Probability of study success relative to a separate analysis of the target study data for the three main treatment effect values considered in the Aprepitant case study ($N_T/2 = 143$). 
     TtP (diff/eq) : test-then-pool with a test for difference/equivalence ($\eta$: significance level of the test. $\lambda$: equivalence margin ). Conditional PP : Conditional Power Prior ($\gamma$: power parameter). p-PP : p-value-based PP ($k$: shape parameter, $\lambda$: equivalence margin). EBPP: Empirical Bayes PP.
RMP : Robust Mixture Prior ($w$: weight of the informative prior component). NPP : Normalized PP ($\xi_\gamma$ and $\sigma_\gamma$ are respectively the mean and standard deviation of the Beta prior on the power parameter $\gamma$). Com. PP : Commensurate PP ($\tau$: heterogeneity parameter). Separate : separate analysis of the target trial data alone.} \label{fig:aprepitant_relative_success_proba_forest_plot_target_sample_size_per_arm_143}
 \end{figure}

\end{document}
